# Supplementary material for: New Tests of Uniformity on the Compact Classical Groups as Diagnostics for Weak-star Mixing of Markov Chains
Source: arXiv:1612.03233 source file (2018-02-25)
Supplement: Supplementary file 1 [file Supplement.pdf]

SUPPLEMENTARY MATERIAL

" **Supplement to "New Tests of Uniformity on the Compact Classical Groups as Diagnostics for Weak-$^*$ Mixing of Markov Chains"**
(doi: 10.1214/00-AOASXXXXSUPP; .pdf). We provide additional supporting material including background and proofs from representation theory, proofs of some of the results, introdcution to Le Cam's theory, further derivation and analysis of local properties, as well as a test based on the trace. The motivating example is also reviewed.

**1. Background on representation theory of Lie groups.** Let $G$ be the group $SO(2n+1)$. A representation $\pi$ of $G$ on a finite-dimensional vector space $V$, denoted by $(\pi, V)$, is a map $\pi : G \to End(V)$ that preserves multiplication. Throughout this text, $V$ is assumed to be finite-dimensional. That is, $\pi(g)$ is a linear operator on $V$ for any $g \in G$, and for all $g, h \in G$

$$\pi(g \cdot h) = \pi(g)\pi(h).$$

This is just an embedding of the group $G$ into space of linear maps on $V$ such that the group multiplication corresponds to composition of linear maps, i.e. to matrix multiplication.

A representation is called reducible if $\pi(g)$ can be decomposed in a block-diagonal form

$$\pi(g) = \begin{bmatrix} \pi_1(g) & 0 \\ 0 & \pi_2(g) \end{bmatrix},$$

for maps $\pi_1, \pi_2$ and all $g$. It is called *irreducible* if it is not reducible. For a compact Lie group $G$, for $SO(2n+1)$ in particular, there are countably many non-equivalent irreducible representations. Moreover, they can be assumed to be unitary in the sense that $\pi(g)$ is a unitary matrix for all $g$. All the representations appearing in this paper are assumed to be unitary.

The character corresponding to a representation $(\pi, V)$ is defined as

$$\chi(g) = \mathrm{tr}(\pi(g)).$$

Characters are invariant under conjugation: $\chi(g) = \chi(h^{-1}gh)$ for all $g, h \in G$. Two elements $g$ and $h$ are conjugate if and only if they have the same eigenvalues. Therefore, $\chi(g)$ is a symmetric function of the eigenvalues of $g$. The characters characterize the representations in the sense that if $\chi_\pi = \chi_\rho$ for two representations $\pi$ and $\rho$, then $\pi = \rho$. The characters corresponding to irreducible representations are called *irreducible characters.* A function on $G$ is called a class function if it is invariant under conjugation. Let $\mathcal{L}^2_{class}(G)$ be

the space of square-integrable class functions on $G$. The following theorems are of fundamental importance (see (Bump, 2004, ch. 4)).

PROPOSITION 1.1 (The Peter-Weyl theorem). *Let* $\{(\pi^\lambda, V^\lambda) \mid \lambda \in \mathcal{I}\}$ *be the set of all distinct irreducible representations of* $G$. *Let* $d_\lambda = \dim V^\lambda$, *and* $\pi^\lambda_{ij}$ *be the* $(i,j)$*-th coordinate of* $\pi^\lambda$. *Then,* $\{\sqrt{d_\lambda}\pi^\lambda_{ij} \mid i, j \leq d_\lambda,\ \lambda \in \mathcal{I}\}$ *is an orthonormal basis for* $\mathcal{L}^2(G)$.

PROPOSITION 1.2 (The Peter-Weyl theorem for characters). *The irreducible characters of* $G$ *form an orthonormal basis for* $\mathcal{L}^2_{class}(G)$.

**2. The Cauchy identity for the characters of compact classical groups.** The Cauchy identity is a well-known result about characters of the unitary group. For two sets of variables, $x_1, \ldots, x_n$ and $y_1, \ldots, y_m$, the Cauchy identity asserts that

$$\sum_\lambda s_\lambda(x_1, \ldots, x_n) s_\lambda(y_1, \ldots, y_m) = \prod_{i,j} \frac{1}{1 - x_i y_j}, \tag{1}$$

where the sum is over all partitions $\lambda$ of all non-negative integers and $s_\lambda$ is the Schur polynomial. The special case of $m = n$ is of particular interest here. Schur polynomials are related to characters of unitary groups in the following way: Let $g \in U(n)$ with eigenvalues $\alpha_1, \ldots, \alpha_n$ and $\lambda$ be a partition with at most $n$ parts. Then,

$$\chi_\lambda(g) = s_\lambda(\alpha_1, \ldots, \alpha_n),$$

where $\chi_\lambda$ is the irreducible character corresponding to $\lambda$. Thus, the representation theoretical version of the Cauchy identity can be written as

$$\sum_\lambda \chi_\lambda(g)\chi_\lambda(h) = \prod_{i=1}^n \prod_{j=1}^n \frac{1}{1 - \alpha_i \beta_j}, \tag{2}$$

where $g \in U(n)$ has eigenvalues $\alpha_1, \ldots, \alpha_n$ and $h \in U(n)$ has eigenvalues $\beta_1, \ldots, \beta_n$. Homogeneity of Schur polynomials yields

$$\sum_\lambda z^{|\lambda|}\chi_\lambda(g)\chi_\lambda(h) = \prod_{i=1}^n \prod_{j=1}^n \frac{1}{1 - z\alpha_i \beta_j} \tag{3}$$

for any $0 < z < 1$.

The Cauchy identity (2) has a conceptual interpretation and generalization from a representation theoretical point of view. This is sketched briefly following Bump (2004, ch. 38). Let $\mathrm{Mat}_n(\mathbb{C})$ be the set of all $n \times n$ complex matrices and $\Sigma^\circ$, the ring of polynomials on $\mathrm{Mat}_n(\mathbb{C})$. Define the action $\Pi^\circ$ of $U(n) \times U(n)$ on $\Sigma^\circ$ as follows. For $(g, h) \in U(n) \times U(n)$ and $f \in \Sigma^\circ$ define

$$\left(\Pi^\circ(g,h)f\right)(x) = f(g^t x h).$$

Then, as a $U(n) \times U(n)$ representation, $\Pi^\circ$ decomposes into irreducible representations as

$$\Pi^\circ \cong \sum_\lambda \pi_\lambda \otimes \pi_\lambda, \tag{4}$$

where $\lambda$ runs through all partitions of length $\leq n$, and $\pi_\lambda$ is the corresponding irreducible representation of $U(n)$. Taking traces on both sides of (4) (in a proper sense of trace for operators on infinite dimensional spaces) yields the Cauchy identity (2). For details of this and an excellent textbook treatment of the Cauchy identity, see Bump (2004, ch. 38). A symmetric function theoretical point of view has been detailed in Macdonald (1995, ch. 1).

2.1. *Type B.* This section gives a Cauchy identity for the compact classical group of type B, i.e. special orthogonal group in odd dimensions. The result for the full orthogonal group, $O(2m+1)$, will follow from this. Before stating the result, recall that irreducible representations of $SO(2m+1)$ are labeled by partitions $\lambda$, of non-negative integers, with at most $m$ parts, see e.g. Proposition 3.1.20 in Goodman and Wallach (2009, ch. 3). Any element $g \in SO(2m+1)$ has an eigenvalue equal to one, and the rest of eigenvalues come in conjugate pairs. The character $so_\lambda$ corresponding to partition $\lambda$ is given explicitly by the Weyl Character Formula (Goodman and Wallach, 2009, ch. 7) as follows:

$$so_\lambda(g) = \frac{\det\left(x_i^{\lambda_j+m-j+\frac{1}{2}} - x_i^{-(\lambda_j+m-j+\frac{1}{2})}\right)}{\det\left(x_i^{m-j+\frac{1}{2}} - x_i^{-(m-j+\frac{1}{2})}\right)}, \tag{5}$$

where $x_1, x_1^{-1}, \ldots, x_m, x_m^{-1}, 1$ are eigenvalues of $g$. We are ready to state our first theorem:

THEOREM 2.1 (CAUCHY IDENTITY FOR $SO(2m+1)$). *Let $so_\lambda$ be the character of $SO(2m+1)$ corresponding to the partition $\lambda$, and $g, h \in SO(2m+$*

1) *with eigenvalues equal to* $x_1, x_1^{-1}, \dots, x_m, x_m^{-1}, 1$ *and* $y_1, y_1^{-1}, \dots, y_m, y_m^{-1}, 1$, *respectively. Then,*

(6)
$$\sum_{\lambda} z^{|\lambda|} so_\lambda(g) so_\lambda(h) = \frac{(1-z)^m \det(C)}{z^{\binom{m}{2}} \prod_{i<j}\left(y_i + y_i^{-1} - (y_j + y_j^{-1})\right) \prod_{i<j}\left(x_i + x_i^{-1} - (x_j + x_j^{-1})\right)}$$

*where* $\lambda$ *runs over all partitions of non-negative integers with at most* $m$ *parts,* $0 < z < 1$ *is an arbitrary parameter and* $C$ *is an* $m \times m$ *matrix defined as*

$$C_{ij} = \frac{(1+z)^2 + z(x_i + x_i^{-1} + y_j + y_j^{-1})}{(1 - zx_iy_j)(1 - zx_i^{-1}y_j)(1 - zx_iy_j^{-1})(1 - zx_i^{-1}y_j^{-1})}.$$

Proof. The proof builds on the classical Cauchy identity in Macdonald (1995, pg. 34). Let $x_1, \dots, x_m$ and $y_1, \dots, y_m$ be two sets of variables. Consider the matrix $X$ defined as

$$X_{ij} = \sum_{k \geq 0} z^k (x_i^{k+\frac{1}{2}} - x_i^{-(k+\frac{1}{2})})(y_j^{k+\frac{1}{2}} - y_j^{-(k+\frac{1}{2})}).$$

The $(i,j)$ entry, $X_{ij}$, can be simplified as follows

$$\begin{aligned} X_{ij} &= \sum_k z^k (x_i^{k+\frac{1}{2}} - x_i^{-(k+\frac{1}{2})})(y_j^{k+\frac{1}{2}} - y_j^{-(k+\frac{1}{2})}) \\ &= x_i^{\frac{1}{2}} y_j^{\frac{1}{2}} \sum_k z^k x_i^k y_j^k - x_i^{\frac{-1}{2}} y_j^{\frac{1}{2}} \sum_k z^k x_i^{-k} y_j^k - x_i^{\frac{1}{2}} y_j^{\frac{-1}{2}} \sum_k z^k x_i^k y_j^{-k} + x_i^{\frac{-1}{2}} y_j^{\frac{-1}{2}} \sum_k z^k x_i^{-k} y_j^{-k} \\ &= \frac{x_i^{\frac{1}{2}} y_j^{\frac{1}{2}}}{1 - zx_iy_j} - \frac{x_i^{\frac{-1}{2}} y_j^{\frac{1}{2}}}{1 - zx_i^{-1}y_j} - \frac{x_i^{\frac{1}{2}} y_j^{\frac{-1}{2}}}{1 - zx_iy_j^{-1}} + \frac{x_i^{\frac{-1}{2}} y_j^{\frac{-1}{2}}}{1 - zx_i^{-1}y_j^{-1}}, \end{aligned}$$

which simplifies to

(7)
$$X_{ij} = \frac{(x_i^{\frac{1}{2}} - x_i^{\frac{-1}{2}})(y_j^{\frac{1}{2}} - y_j^{\frac{-1}{2}})(1-z)[(1+z)^2 + z(x_i + x_i^{-1} + y_j + y_j^{-1})]}{(1 - zx_iy_j)(1 - zx_i^{-1}y_j)(1 - zx_iy_j^{-1})(1 - zx_i^{-1}y_j^{-1})}.$$

This shows the relation between $X$ and the determinant on the right hand side of identity (6). Now expand $\det(X)$ as follows

$$\det(X) = \det\left(\sum_{k\geq 0} z^k (x_i^{k+\frac{1}{2}} - x_i^{-(k+\frac{1}{2})})(y_j^{k+\frac{1}{2}} - y_j^{-(k+\frac{1}{2})})\right)$$
$$= \sum_{\pi\in S_m} sign(\pi) \prod_{i\leq m}\left(\sum_{k\geq 0} z^k (x_i^{k+\frac{1}{2}} - x_i^{-(k+\frac{1}{2})})(y_{\pi(i)}^{k+\frac{1}{2}} - y_{\pi(i)}^{-(k+\frac{1}{2})})\right).$$

Expanding the product on the right hand side leads to

$$\det(X) = \sum_{\pi\in S_m} sign(\pi) \sum_{a_1,a_2,\ldots,a_m\geq 0} \prod_{i\leq m} z^{a_i}\left((x_i^{a_i+\frac{1}{2}} - x_i^{-(a_i+\frac{1}{2})})(y_{\pi(i)}^{a_i+\frac{1}{2}} - y_{\pi(i)}^{-(a_i+\frac{1}{2})})\right).$$

Changing the order of summation and using the definition of $m\times m$ determinants yields

$$\det(X) = \sum_{a_1,a_2,\ldots,a_m\geq 0} z^{\sum_i a_i} \sum_{\pi\in S_m} sign(\pi) \prod_{i\leq m}\left((x_i^{a_i+\frac{1}{2}} - x_i^{-(a_i+\frac{1}{2})})(y_{\pi(i)}^{a_i+\frac{1}{2}} - y_{\pi(i)}^{-(a_i+\frac{1}{2})})\right)$$
$$= \sum_{a\in\mathbb{Z}_+^m} z^{|a|} \det\left((x_i^{a_i+\frac{1}{2}} - x_i^{-(a_i+\frac{1}{2})})(y_j^{a_i+\frac{1}{2}} - y_j^{-(a_i+\frac{1}{2})})\right)$$
$$= \sum_{a\in\mathbb{Z}_+^m} z^{|a|} \det\left(y_j^{a_i+\frac{1}{2}} - y_j^{-(a_i+\frac{1}{2})}\right) \prod_i (x_i^{a_i+\frac{1}{2}} - x_i^{-(a_i+\frac{1}{2})}).$$

The last equality can be rewritten as follows by ordering the $m$-tuple $a\in\mathbb{Z}^m$.

$$\det(X) = \sum_{a_1\geq\ldots\geq a_m\geq 0} \sum_{\sigma\in S_m} z^{|a|} \det\left(y_j^{a_i+\frac{1}{2}} - y_j^{-(a_i+\frac{1}{2})}\right) sign(\sigma) \prod_i (x_i^{a_{\sigma(i)}+\frac{1}{2}} - x_i^{-(a_{\sigma(i)}+\frac{1}{2})})$$
$$= \sum_{a_1\geq\ldots\geq a_m\geq 0} z^{|a|} \det\left(y_j^{a_i+\frac{1}{2}} - y_j^{-(a_i+\frac{1}{2})}\right) \sum_{\sigma\in S_m} sign(\sigma) \prod_i (x_i^{a_{\sigma(i)}+\frac{1}{2}} - x_i^{-(a_{\sigma(i)}+\frac{1}{2})})$$
$$= \sum_{a_1\geq\ldots\geq a_m\geq 0} z^{|a|} \det\left(y_j^{a_i+\frac{1}{2}} - y_j^{-(a_i+\frac{1}{2})}\right) \det\left(x_j^{a_i+\frac{1}{2}} - x_j^{-(a_i+\frac{1}{2})}\right).$$

Note that if two of $a_i$'s are equal then both determinants on the right hand side are zero. Thus, it may be assumed that $a_1 > a_2 > \ldots > a_m \geq 0$.

This is equivalent to the condition that $a_i - (m-i)$ is a non-increasing sequence. Define $\lambda_i = a_i - m + i$, then $\lambda_1 \geq \ldots \geq \lambda_m \geq 0$. The last equality translates to the following in terms of $\lambda$:

$$\det(X) = \sum_{\lambda_1 \geq \ldots \geq \lambda_m \geq 0} z^{|\lambda| + \binom{m}{2}} \det\left(A^\lambda\right) \det\left(B^\lambda\right),$$
$$A^\lambda_{i,j} = y_j^{\lambda_i + m - i + \frac{1}{2}} - y_j^{-(\lambda_i + m - i + \frac{1}{2})},$$
$$B^\lambda_{i,j} = x_j^{\lambda_i + m - i + \frac{1}{2}} - x_j^{-(\lambda_i + m - i + \frac{1}{2})}.$$

Assume $x_1, \ldots, x_m$ and $y_1, \ldots, y_m$ are such that there exist $g, h \in SO(2m+1)$ with eigenvalues equal to $x_1, x_1^{-1}, \ldots, x_m, x_m^{-1}, 1$ and $y_1, y_1^{-1}, \ldots, y_m, y_m^{-1}, 1$, respectively. Dividing by a factor of the following form

$$z^{\binom{m}{2}} \det\left(y_j^{m-i+\frac{1}{2}} - y_j^{-(m-i+\frac{1}{2})}\right) \det\left(x_j^{m-i+\frac{1}{2}} - x_j^{-(m-i+\frac{1}{2})}\right),$$

and using the Weyl character formula yields

(8)
$$\sum_\lambda z^{|\lambda|} so_\lambda(g) so_\lambda(h) = \frac{z^{-\binom{m}{2}} \det(X)}{\det\left(y_j^{m-i+\frac{1}{2}} - y_j^{-(m-i+\frac{1}{2})}\right) \det\left(x_j^{m-i+\frac{1}{2}} - x_j^{-(m-i+\frac{1}{2})}\right)},$$

where $\lambda$ runs over all partitions of an arbitrary integer with at most $m$ parts. To finish the proof, the right side of (8) is simplified; from (7),

$$\det(X) = \det\left(\frac{(x_i^{\frac{1}{2}} - x_i^{\frac{-1}{2}})(y_j^{\frac{1}{2}} - y_j^{\frac{-1}{2}})(1-z)[(1+z)^2 + z(x_i + x_i^{-1} + y_j + y_j^{-1})]}{(1 - z x_i y_j)(1 - z x_i^{-1} y_j)(1 - z x_i y_j^{-1})(1 - z x_i^{-1} y_j^{-1})}\right)$$
$$= (1-z)^m \prod_i (x_i^{\frac{1}{2}} - x_i^{\frac{-1}{2}})(y_i^{\frac{1}{2}} - y_i^{\frac{-1}{2}}) \det(C),$$

where $C$ is defined in the statement of the theorem. To get to the final form, one more simplification is needed. Note that

$$x_j^{m-i+\frac{1}{2}} - x_j^{-(m-i+\frac{1}{2})} = (x_j^{\frac{1}{2}} - x_j^{\frac{-1}{2}})(x_j^{m-i} + x_j^{m-i-1} + \ldots + x_j^{-(m-i)})$$

leads to

$$\det\left(x_j^{m-i+\frac{1}{2}} - x_j^{-(m-i+\frac{1}{2})}\right) = \det\left(x_j^{m-i} + x_j^{m-i-1} + \ldots + x_j^{-(m-i)}\right) \prod_{1 \leq j \leq m} (x_j^{\frac{1}{2}} - x_j^{\frac{-1}{2}}).$$

Subtracting $(i+1)^{th}$ row from the $i^{th}$ row for $i = 1, 2, \dots, m-1$ yields

$$\begin{aligned}
\det\left(x_j^{m-i+\frac{1}{2}} - x_j^{-(m-i+\frac{1}{2})}\right) &= \det\left(x_j^{m-i} + x_j^{-(m-i)}\right) \prod_{1\le j\le m} (x_j^{\frac{1}{2}} - x_j^{\frac{-1}{2}}) \\
&= \det\left((x_j + x_j^{-1})^{m-i}\right) \prod_{1\le j\le m} (x_j^{\frac{1}{2}} - x_j^{\frac{-1}{2}}) \\
&= \prod_{i<j}(x_i + x_i^{-1} - (x_j + x_j^{-1})) \prod_{1\le j\le m} (x_j^{\frac{1}{2}} - x_j^{\frac{-1}{2}}),
\end{aligned}$$

where the second equality can be proved by simple row operations, and the last equality is the Vandermonde identity. Simplification of the determinant involving $y$ is identical to the calculations above. Substituting these simplifications in (8) proves the theorem. □

REMARK 2.2. *It is noteworthy that unlike the unitary group, the characters $o_\lambda$ of the orthogonal group are not homogeneous functions of the eigenvalues. This perhaps is the reason that the Cauchy identity is much more complicated for the orthogonal group than for the unitary group.*

*With Theorem 2.1 in hand, a Cauchy identity for the orthogonal group $O(2m+1)$ is a straightforward corollary .*

COROLLARY 2.3 (CAUCHY IDENTITY FOR $O(2m+1)$). *Let $o_\lambda$ be the character of $O(2m+1)$ corresponding to the partition $\lambda$, and $g, h \in O(2m+1)$ with eigenvalues equal to $x_1, x_1^{-1}, \dots, x_m, x_m^{-1}, det(g)$ and $y_1, y_1^{-1}, \dots, y_m, y_m^{-1}, det(h)$, respectively, then*

(9)
$$\sum_\lambda z^{|\lambda|} o_\lambda(g) o_\lambda(h) = \frac{(1-det(gh)z)^m det\left(\frac{(1+det(gh)z)^2 + z(det(h)(x_i+x_i^{-1}) + det(g)(y_j+y_j^{-1}))}{(1-zx_iy_j)(1-zx_i^{-1}y_j)(1-zx_iy_j^{-1})(1-zx_i^{-1}y_j^{-1})}\right)}{z^{\binom{m}{2}} \prod_{i<j}\left(y_i + y_i^{-1} - (y_j + y_j^{-1})\right) \prod_{i<j}\left(x_i + x_i^{-1} - (x_j + x_j^{-1})\right)},$$

*where $\lambda$ runs over all partitions of arbitrary integers with at most $m$ parts.*

PROOF. Let $n = 2m+1$. Recall that the irreducible representations of $O(n)$ are labeled by partitions $\lambda$ of arbitrary non-negative integers for which $\lambda_1' + \lambda_2' \le n$, where $\lambda'$ is the transpose of $\lambda$ defined as $\lambda_i' = \#\{j : \lambda_j \ge i\}$ (see Goodman and Wallach (2009, ch. 10)). For a partition $\lambda$ with $\lambda_1' \le m$, define $\tilde{\lambda}$ as the partition with $\tilde{\lambda}' = (n - \lambda_1', \lambda_2', ..., \lambda_l')$. For each partition $\lambda$ with $\lambda_1' \le m$, there exist an irreducible representation of $O(n)$ labeled by $\lambda$

and one labeled with $\tilde{\lambda}$. Moreover, the Weyl character formula asserts that

$$o_\lambda(g) = \frac{\det\left(x_i^{\lambda_j+m-j+\frac{1}{2}} - det(g)x_i^{-(\lambda_j+m-j+\frac{1}{2})}\right)}{\det\left(x_i^{m-j+\frac{1}{2}} - det(g)x_i^{-(m-j+\frac{1}{2})}\right)},$$
$$o_{\tilde{\lambda}}(g) = det(g)o_\lambda(g).$$

The last equality justifies summing only over $\lambda$ with at most $m$ parts. The rest of the proof is identical to that in Theorem 2.1. □

2.1.1. *Limit as* $z \to 1$. The Identity (6) exhibits interesting limiting behavior as $z$ tends to 1. Assume throughout this section that $g$ and $h$ share no common eigenvalues. The right hand side is equal to zero at $z = 1$, but the left hand side does not converge at $z = 1$, because the series defining $X_{i,j}$ do not converge. However, under an extended notion of series convergence, i.e. Cesaro $C_\alpha$-summability, the left hand side converges to a limit at $z = 1$ which coincides with the value of the right hand side.

DEFIN 2.4 ($C_k$-summability). *Given a sequence* $\{a_n\}$, *define*

$$A_n^{(-1)} = a_n, \quad A_n^{(k)} = \sum_{i=1}^{n} A_i^{(k-1)} \quad k = 1, 2, \dots .$$

*Let* $E_n^{(\alpha)}$ *be the corresponding sequence* $A_n^{(\alpha)}$ *starting from the initial sequence* $e_1 = 1, e_i = 0$ *for* $i > 1$ . *The series* $\sum_n a_n$ *is called* $C_\alpha$*-summable to the value* $s$ *if*

$$\lim_{n\to\infty} \frac{A_n^{(\alpha)}}{E_n^{(\alpha)}} = s.$$

It is known that the geometric series $1 + z + z^2 + \dots$ is $C_1$-summable for $|z| = 1,\ z \neq 1$ with $C_1$-limit $\frac{1}{1-z}$. This ensures that the entries $X_{i,j}$ of the matrix $X$ are $C_1$-summable to their corresponding closed forms given in (7). Then, the following lemma implies that all the terms in the expansion of $\det(X)$ are $C_{2m-1}$-summable. Therefore, the left hand side of (6) is $C_{2m-1}$-summable at $z = 1$.

LEMMA 2.5 (Theorem 277 in Knopp (1948)). *If* $\sum a_n$ *is* $C_\alpha$*-summable to the value* $A$ *and* $\sum b_n$ *is* $C_\beta$*-summable to the value* $B$, *then their Cauchy product,*

$$\sum c_n = \sum (a_0 b_n + a_1 b_{n-1} + \dots + a_n b_0),$$

*is certainly $C_\gamma$-summable to the value $C = AB$, where $\gamma = \alpha + \beta + 1$.*

The following lemma justifies taking the limit $z \to 1$ on both sides of (6). This, together with the discussion above, imply that, for $z \to 1$, the left hand side converges to the value of the right hand side which is equal to zero.

LEMMA 2.6 (Theorem 278 in Knopp (1948)). *If a power series $f(z) = \sum a_n z^n$ has convergence radius 1 and is $C_k$-summable to the value $s$ at the point $z = 1$, then*

$$f(z) \to s$$

*for every mode of approach of $z$ to 1, in which $z$ remains within an angle of vertex $+1$, bounded by two fixed chords of the unit circle. This certainly includes the case $z \to 1$ for $z \in [0, 1]$.*

MacPhail (1941) proved that the series $\sum_n P(n)e^{in\theta}$ is $C_k$-summable for any polynomial $P$ of degree less than $k$. This allows differentiating both sides of identity (6) with respect to $z$. More precisely, write identity (6) as

$$\sum_\lambda z^{\binom{m}{2}+|\lambda|} so_\lambda(g) so_\lambda(h) = \frac{(1-z)^m \det(C)}{\prod_{i<j}\left(y_i + y_i^{-1} - (y_j + y_j^{-1})\right)\prod_{i<j}\left(x_i + x_i^{-1} - (x_j + x_j^{-1})\right)}.$$

Differentiating $m$ times with respect to $z$ yields

$$\sum_\lambda \frac{(\binom{m}{2} + |\lambda|)!}{(\binom{m}{2} + |\lambda| - m)!} z^{\binom{m}{2}+|\lambda|-m} so_\lambda(g) so_\lambda(h)$$
$$= \frac{\frac{\partial^m}{\partial z^m}\left[(1-z)^m \det(C)\right]}{\prod_{i<j}\left(y_i + y_i^{-1} - (y_j + y_j^{-1})\right)\prod_{i<j}\left(x_i + x_i^{-1} - (x_j + x_j^{-1})\right)}.$$

Note that the left hand side is Cesaro summable at $z = 1$ to the value of the right hand side at $z = 1$. This follows from the Leibniz rule, Cesaro summablity of the derivatives of geometric series, and lemma 2.5 using an argument similar to the one above. Then, applying lemma 2.6, and simplification of the right hand side, yields

(10)
$$\lim_{z\to 1} \sum_\lambda \binom{\binom{m}{2} + |\lambda|}{m} z^{\binom{m}{2}+|\lambda|-m} so_\lambda(g) so_\lambda(h) = \frac{(-1)^m \det\left(\frac{u_i+v_j}{(u_i-v_j)^2}\right)}{\prod_{i<j}(u_i - u_j)\prod_{i<j}(v_i - v_j)},$$

where $u_i = x_i + x_i^{-1} + 2$ and $v_j = y_j + y_j^{-1} + 2$, and the limit is taken over real number $z \in (0, 1)$ approaching 1. This suggests using the right hand side of (10) for computational purposes.

2.2. *Type C.* The type C root system corresponds to the compact (real) *symplectic* group. The statement and proof of the type C Cauchy identity is very similar to that of type B. Irreducible representations of the symplectic group of order $m$, $Sp(2m)$, are labeled by partitions $\lambda$, of non-negative integers, with at most $m$ parts (see Proposition 3.1.20 in Goodman and Wallach (2009, ch. 3)). Let $g \in Sp(2m)$ have eigenvalues $x_1, x_1^{-1}, \ldots, x_m, x_m^{-1}$. The character $sp_\lambda$ corresponding to partition $\lambda$ is given explicitly by the Weyl Character Formula:

$$sp_\lambda(g) = \frac{\det\left(x_i^{\lambda_j+m-j+1} - x_i^{-(\lambda_j+m-j+1)}\right)}{\det\left(x_i^{m-j+1} - x_i^{-(m-j+1)}\right)}. \tag{11}$$

With this notation, the main result of this section is:

THEOREM 2.7 (CAUCHY IDENTITY FOR $Sp(2m)$). *Let $sp_\lambda$ be the character of $Sp(2m)$ corresponding to the partition $\lambda$, and $g, h \in Sp(2m)$ with eigenvalues equal to $x_1, x_1^{-1}, \ldots, x_m, x_m^{-1}$ and $y_1, y_1^{-1}, \ldots, y_m, y_m^{-1}$, respectively. Then,*

(12)

$$\sum_\lambda z^{|\lambda|} sp_\lambda(g)\, sp_\lambda(h) = \frac{(1-z^2)^m \det\left(\frac{1}{(1-zx_iy_j)(1-zx_i^{-1}y_j)(1-zx_iy_j^{-1})(1-zx_i^{-1}y_j^{-1})}\right)}{z^{\binom{m}{2}} \prod_{i<j}\left(y_i + y_i^{-1} - (y_j + y_j^{-1})\right) \prod_{i<j}\left(x_i + x_i^{-1} - (x_j + x_j^{-1})\right)}$$

*where $\lambda$ runs over all partitions of non-negative integers with at most $m$ parts and $0 < z < 1$ is an arbitrary parameter.*

REMARK 2.8. *The author was informed by Dr. Wheeler that the Cauchy indentity stated above for the symplectic group was independently proved in (Wheeler and Zinn-Justin, 2016).*

PROOF. Let $x_1, \ldots, x_m$ and $y_1, \ldots, y_m$ be two sets of variables. Consider the matrix $X$ defined as

$$X_{ij} = \sum_{k\geq 0} z^k (x_i^{k+1} - x_i^{-(k+1)})(y_j^{k+1} - y_j^{-(k+1)}).$$

Write

$$X_{ij} = \frac{(1-z^2)(x_i - x_i^{-1})(y_j - y_j^{-1})}{(1-zx_iy_j)(1-zx_i^{-1}y_j)(1-zx_iy_j^{-1})(1-zx_i^{-1}y_j^{-1})}. \tag{13}$$

Expand $\det(X)$ as follows

$$\det(X) = \det\left(\sum_{k\geq 0} z^k (x_i^{k+1} - x_i^{-(k+1)})(y_j^{k+1} - y_j^{-(k+1)})\right)$$
$$= \sum_{\pi\in S_m} sign(\pi) \prod_{i\leq m}\left(\sum_{k\geq 0} z^k (x_i^{k+1} - x_i^{-(k+1)})(y_{\pi(i)}^{k+1} - y_{\pi(i)}^{-(k+1)})\right).$$

Expanding the product on the right hand side leads to

$$\det(X) = \sum_{\pi\in S_m} sign(\pi) \sum_{a_1,a_2,\dots,a_m\geq 0} \prod_{i\leq m} z^{a_i}\left((x_i^{a_i+1} - x_i^{-(a_i+1)})(y_{\pi(i)}^{a_i+1} - y_{\pi(i)}^{-(a_i+1)})\right).$$

Changing the order of summation and using the definition of $m\times m$ determinant yields

$$\det(X) = \sum_{a_1,a_2,\dots,a_m\geq 0} z^{\sum_i a_i} \sum_{\pi\in S_m} sign(\pi)\prod_{i\leq m}\left((x_i^{a_i+1} - x_i^{-(a_i+1)})(y_{\pi(i)}^{a_i+1} - y_{\pi(i)}^{-(a_i+1)})\right)$$
$$= \sum_{a\in\mathbb{Z}_+^m} z^{|a|}\det\left(y_j^{a_i+1} - y_j^{-(a_i+1)}\right)\prod_i (x_i^{a_i+1} - x_i^{-(a_i+1)}).$$

Rewrite the last equality as follows by ordering the $m$-tuple $a\in\mathbb{Z}^m$.

$$\det(X) = \sum_{a_1\geq\dots\geq a_m\geq 0}\sum_{\sigma\in S_m} z^{|a|}\det\left(y_j^{a_i+1} - y_j^{-(a_i+1)}\right) sign(\sigma)\prod_i (x_i^{a_{\sigma(i)}+1} - x_i^{-(a_{\sigma(i)}+1)})$$
$$= \sum_{a_1\geq\dots\geq a_m\geq 0} z^{|a|}\det\left(y_j^{a_i+1} - y_j^{-(a_i+1)}\right)\det\left(x_j^{a_i+1} - x_j^{-(a_i+1)}\right).$$

If two of $a_i$'s are equal then both determinants on RHS are zero. Thus, assume $a_1 > a_2 > \dots > a_m \geq 0$. Define $\lambda_i = a_i - m + i$, then $\lambda_1\geq\dots\geq\lambda_m\geq 0$. The last equality translates to the following in terms of $\lambda$:

$$\det(X) = \sum_{\lambda_1\geq\dots\geq\lambda_m\geq 0} z^{|\lambda|+\binom{m}{2}}\det\left(A^\lambda\right)\det\left(B^\lambda\right),$$
$$A_{i,j}^\lambda = y_j^{\lambda_i+m-i+1} - y_j^{-(\lambda_i+m-i+1)},$$
$$B_{i,j}^\lambda = x_j^{\lambda_i+m-i+1} - x_j^{-(\lambda_i+m-i+1)}.$$

Assume $x_1, \dots, x_m$ and $y_1, \dots, y_m$ are such that there exist $g, h \in Sp(2m)$ with eigenvalues equal to $x_1, x_1^{-1}, \dots, x_m, x_m^{-1}$ and $y_1, y_1^{-1}, \dots, y_m, y_m^{-1}$, respectively. Dividing by a factor of the following form

$$z^{\binom{m}{2}} \det\left(y_j^{m-i+1} - y_j^{-(m-i+1)}\right) \det\left(x_j^{m-i+1} - x_j^{-(m-i+1)}\right),$$

and using the Weyl character formula yields

(14)

$$\sum_\lambda z^{|\lambda|} sp_\lambda(g) sp_\lambda(h) = \frac{z^{-\binom{m}{2}} \det(X)}{\det\left(y_j^{m-i+1} - y_j^{-(m-i+1)}\right) \det\left(x_j^{m-i+1} - x_j^{-(m-i+1)}\right)},$$

where $\lambda$ runs over all partitions of an arbitrary integer with at most $m$ parts. Using equation (13)

$$\begin{aligned}\det(X) &= \det\left(\frac{(x_i - x_i^{-1})(y_j - y_j^{-1})(1 - z^2)}{(1 - zx_iy_j)(1 - zx_i^{-1}y_j)(1 - zx_iy_j^{-1})(1 - zx_i^{-1}y_j^{-1})}\right) \\ &= (1 - z^2)^m \prod_i (x_i - x_i^{-1})(y_i - y_i^{-1}) \det\left(\frac{1}{(1 - zx_iy_j)(1 - zx_i^{-1}y_j)(1 - zx_iy_j^{-1})(1 - zx_i^{-1}y_j^{-1})}\right)\end{aligned}$$

To get to the final form, one more simplification is needed. Note that

$$x_j^{m-i+1} - x_j^{-(m-i+1)} = (x_j - x_j^{-1})(x_j^{m-i} + x_j^{m-i-2} + \dots + x_j^{-(m-i)})$$

leads to

$$\det\left(x_j^{m-i+1} - x_j^{-(m-i+1)}\right) = \det\left(x_j^{m-i} + x_j^{m-i-2} + \dots + x_j^{-(m-i)}\right) \prod_{1 \le j \le m} (x_j - x_j^{-1}).$$

Subtracting $(i+2)^{th}$ row from the $i^{th}$ row for $i = 1, 2, \dots, m-2$ yields

$$\begin{aligned}\det\left(x_j^{m-i+1} - x_j^{-(m-i+1)}\right) &= \det\left(x_j^{m-i} + x_j^{-(m-i)}\right) \prod_{1 \le j \le m} (x_j - x_j^{-1}) \\ &= \det\left((x_j + x_j^{-1})^{m-i}\right) \prod_{1 \le j \le m} (x_j - x_j^{-1}) \\ &= \prod_{i<j} (x_i + x_i^{-1} - (x_j + x_j^{-1})) \prod_{1 \le j \le m} (x_j - x_j^{-1}).\end{aligned}$$

Substituting these simplifications in (14) proves the theorem. □

2.3. *Type D.* The situation is more subtle for type D, which corresponds to the special orthogonal groups in even dimensions. Focus on $SO(2m)$. The irreducible representations of $SO(2m)$ are indexed by sequences of integers $\lambda = (\lambda_1, \lambda_2, ..., \lambda_m)$ and $\lambda^- = (\lambda_1, \lambda_2, ..., \lambda_{m-1}, -\lambda_m)$, where $\lambda$ is a partition with at most $m$ parts. The Weyl character formula is as follows. Let $x_1, x_1^{-1}, \ldots, x_m, x_m^{-1}$ are eigenvalues of $g \in SO(2m)$. If $\tilde{\lambda}_1 < m$ , i.e. $\lambda_m = 0$, then

$$so_\lambda(g) = \frac{\det\left(x_i^{\lambda_j+m-j} + x_i^{-(\lambda_j+m-j)}\right)}{\det\left(x_i^{m-j} + x_i^{-(m-j)}\right)}. \tag{15}$$

If $\tilde{\lambda}_1 = m$, i.e. $\lambda_m > 0$, then the character of the irreducible representation corresponding to $\lambda$ is given by

$$so_\lambda(g) = \frac{\det\left(x_i^{\lambda_j+m-j} + x_i^{-(\lambda_j+m-j)}\right) - \det\left(x_i^{\lambda_j+m-j} - x_i^{-(\lambda_j+m-j)}\right)}{2\det\left(x_i^{m-j} + x_i^{-(m-j)}\right)}, \tag{16}$$

and the one corresponding to $\lambda^-$ is given as

$$so_{\lambda^-}(g) = \frac{\det\left(x_i^{\lambda_j+m-j} + x_i^{-(\lambda_j+m-j)}\right) + \det\left(x_i^{\lambda_j+m-j} - x_i^{-(\lambda_j+m-j)}\right)}{2\det\left(x_i^{m-j} + x_i^{-(m-j)}\right)}. \tag{17}$$

Define $\chi_\lambda$ as $so_\lambda$ if $\tilde{\lambda}_1 < m$, and as $so_\lambda + so_{\lambda^-}$ if $\tilde{\lambda}_1 = m$. Note that $\chi_\lambda$ is the restriction of the irreducible character of $O(2m)$ to $SO(2m)$; it is an irreducible character of $SO(2m)$ if and only if $\tilde{\lambda}_1 < m$. We will state the Cauchy identity in terms of $\{\chi_\lambda\}$.

THEOREM 2.9 (CAUCHY IDENTITY FOR $SO(2m)$). *Let $\chi_\lambda$ be as above, and $g, h \in SO(2m)$ with eigenvalues equal to $x_1, x_1^{-1}, \ldots, x_m, x_m^{-1}$ and $y_1, y_1^{-1}, \ldots, y_m, y_m^{-1}$, respectively. Then,*

$$\sum_\lambda z^{|\lambda|}\chi_\lambda(g)\chi_\lambda(h) = \frac{\det\left(\frac{1}{1-zx_iy_j} + \frac{1}{1-zx_i^{-1}y_j} + \frac{1}{1-zx_iy_j^{-1}} + \frac{1}{1-zx_i^{-1}y_j^{-1}}\right)}{z^{\binom{m}{2}}\prod_{i<j}\left(y_i + y_i^{-1} - (y_j + y_j^{-1})\right)\prod_{i<j}\left(x_i + x_i^{-1} - (x_j + x_j^{-1})\right)} \tag{18}$$

*where $\lambda$ runs over all partitions of non-negative integers with at most $m$ parts and $0 < z < 1$ is an arbitrary parameter.*

Proof. Let $x_1, \ldots, x_m$ and $y_1, \ldots, y_m$ be two sets of variables. Consider the matrix $X$ defined as

$$\begin{aligned} X_{ij} &= \sum_{k \geq 0} z^k (x_i^k + x_i^{-k})(y_j^k + y_j^{-k}) \\ &= \frac{1}{1 - zx_iy_j} + \frac{1}{1 - zx_i^{-1}y_j} + \frac{1}{1 - zx_iy_j^{-1}} + \frac{1}{1 - zx_i^{-1}y_j^{-1}}. \end{aligned}$$

Expand $\det(X)$ to get (similar to proof of Theorem 2.1)

$$\begin{aligned} \det(X) &= \det\left( \sum_{k \geq 0} z^k (x_i^k + x_i^{-k})(y_j^k + y_j^{-k}) \right) \\ &= \sum_{\pi \in S_m} sign(\pi) \prod_{i \leq m} \left( \sum_{k \geq 0} z^k (x_i^k + x_i^{-k})(y_{\pi(i)}^k + y_{\pi(i)}^{-k}) \right) \\ &= \sum_{\pi \in S_m} sign(\pi) \sum_{a_1, a_2, \ldots, a_m \geq 0} \prod_{i \leq m} z^{a_i} \left( (x_i^{a_i} + x_i^{-(a_i)})(y_{\pi(i)}^{a_i} + y_{\pi(i)}^{-(a_i)}) \right) \\ &= \sum_{a_1, a_2, \ldots, a_m \geq 0} z^{\sum_i a_i} \sum_{\pi \in S_m} sign(\pi) \prod_{i \leq m} \left( (x_i^{a_i} + x_i^{-(a_i)})(y_{\pi(i)}^{a_i} + y_{\pi(i)}^{-(a_i)}) \right) \\ &= \sum_{a \in \mathbb{Z}_+^m} z^{|a|} \det\left( y_j^{a_i} + y_j^{-(a_i)} \right) \prod_i (x_i^{a_i} + x_i^{-(a_i)}). \end{aligned}$$

Rewrite the last equality as follows by ordering the $m$-tuple $a \in \mathbb{Z}^m$.

$$\det(X) = \sum_{a_1 \geq \ldots \geq a_m \geq 0} z^{|a|} \det\left( y_j^{a_i} + y_j^{-(a_i)} \right) \det\left( x_j^{a_i} + x_j^{-(a_i)} \right).$$

Clearly $a_1 > a_2 > \ldots > a_m \geq 0$. Define $\lambda_i = a_i - m + i$, then $\lambda_1 \geq \ldots \geq \lambda_m \geq 0$. The last equality translates to the following in terms of $\lambda$:

$$\begin{aligned} \det(X) &= \sum_{\lambda_1 \geq \ldots \geq \lambda_m \geq 0} z^{|\lambda| + \binom{m}{2}} \det\left( A^\lambda \right) \det\left( B^\lambda \right), \\ A_{i,j}^\lambda &= y_j^{\lambda_i + m - i} + y_j^{-(\lambda_i + m - i)}, \\ B_{i,j}^\lambda &= x_j^{\lambda_i + m - i} + x_j^{-(\lambda_i + m - i)}. \end{aligned}$$

Assume $x_1, \ldots, x_m$ and $y_1, \ldots, y_m$ are such that there exist $g, h \in SO(2m)$ with eigenvalues equal to $x_1, x_1^{-1}, \ldots, x_m, x_m^{-1}$ and $y_1, y_1^{-1}, \ldots, y_m, y_m^{-1}$, respectively. Dividing by a factor of the following form

$$z^{\binom{m}{2}} \det\left( y_j^{m-i} + y_j^{-(m-i)} \right) \det\left( x_j^{m-i} + x_j^{-(m-i)} \right),$$

and using definition of $\chi_\lambda$ yields

$$\sum_{\lambda} z^{|\lambda|}\chi_\lambda(g)\chi_\lambda(h) = \frac{z^{-\binom{m}{2}}\det(X)}{\det\left(y_j^{m-i}+y_j^{-(m-i)}\right)\det\left(x_j^{m-i}+x_j^{-(m-i)}\right)}, \tag{19}$$

where $\lambda$ runs over all partitions of an arbitrary integer with at most $m$ parts. To get to the final form note that

$$\begin{aligned}\det\left(x_j^{m-i}+x_j^{-(m-i)}\right) &= \det\left((x_j+x_j^{-1})^{m-i}\right)\\ &= \prod_{i<j}(x_i+x_i^{-1}-(x_j+x_j^{-1})).\end{aligned}$$

Substituting these simplifications in (19) proves the theorem. □

REMARK 2.10. *A similar $z \to 1$ analysis of Type C and Type D Cauchy identities is possible and gives rise to similar expressions as in Type B case. Carrying out the details is straightforward and omitted here.*

**3. Facts used in section 4 of the main paper.** Let $\lambda = (\lambda_1, \ldots, \lambda_m)$ be a partition of $n$. It is customary to interpret $\lambda$ graphically as a Young diagram, namely a left-justified array of square cells with $m$ rows and $\lambda_i$ cells in the $i$th row for each $1 \le i \le m$. For each cell of the Young diagram in coordinates $(i, j)$ (that is, the cell in the$i$th row and $j$th column), the hook $H_\lambda(i, j)$ is the set of cells $(a, b)$ such that $a = i$ and $b \ge j$ or $a \ge i$ and $b = j$. The *hook-length* $h_\lambda(i, j)$ is the number of cells in the hook $H_\lambda(i, j)$. For each cell $(i, j)$, the *content* $c_\lambda(i, j)$ of $\lambda$ at $(i, j)$ is $j - i$.

Using the notation above we are ready to state the following fact about the Schur functions, which is the key to some of our formulas.

PROPOSITION 3.1 (Macdonald (1995), page 80). *Let $s_\lambda$ be the Schur function and $q \in [0, 1]$. Then,*

$$s_\lambda(1, q, \ldots, q^{n-1}) = q^{n(\lambda)} \prod_{x\in\lambda} \frac{1-q^{n+c(x)}}{1-q^{h(x)}}, \tag{20}$$

*where $n(\lambda) = \sum_i \binom{\lambda_i'}{2}$, $h(x)$ is the hook length of a partition at $x$, and $c(x)$ is the content of a partition at $x$.*

For a textbook exposition to Fourier analysis and connections to probability measures on Lie groups see Applebaum and Heyer (2014).

3.1. $SO(2n+1)$. The irreducible representations of $SO(2n+1)$ are labeled by partitions of arbitrary non-negative integers with at most $n$ parts. For such a partition $\lambda = (\lambda_1, \dots, \lambda_k)$ the irreducible character corresponding to $\lambda$ is given by the Weyl character formula (Bump, 2004, ch. 22) as

$$\chi_\lambda(g) = \frac{\det\left[e^{i\theta_k(\lambda_l+n-l+\frac{1}{2})} - e^{-i\theta_k(\lambda_l+n-l+\frac{1}{2})}\right]_{k,l}}{\det\left[e^{i\theta_k(n-l+\frac{1}{2})} - e^{-i\theta_k(n-l+\frac{1}{2})}\right]_{k,l}} = \frac{\det\left[\sin\left(\theta_k(\lambda_l+n-l+\frac{1}{2})\right)\right]_{k,l}}{\det\left[\sin\left(\theta_k(n-l+\frac{1}{2})\right)\right]_{k,l}}, \tag{21}$$

where $1, e^{\pm i\theta_1}, \dots, e^{\pm i\theta_n}$ are the eigenvalues of $g$.

PROPOSITION 3.2 (The Cauchy-Littlewood identity Weyl (1946), Section 7.9). *Let $\chi_\lambda$ be the irreducible character of $G = SO(2n+1)$ and $s_\lambda$ the Schur function of symmetric function theory. Let $g \in G$ with eigenvalues $1, e^{\pm i\theta_1}, \dots, e^{\pm i\theta_n}$. Then,*

$$\sum_\lambda s_\lambda(x_1,\dots,x_n)\chi_\lambda(g) = \frac{\prod_{k<j}(1-x_kx_j)\prod_k(1+x_k)}{\prod_{k,j}(1-x_ke^{i\theta_j})(1-x_ke^{-i\theta_j})}. \tag{22}$$

Therefore, substituting $x_k = z\cdot q^{k-1}$ in (22) yields

$$\sum_{\lambda\neq 0} c_\lambda(z,q)\chi_\lambda(g) = \frac{\prod_{k<j}(1-z^2q^{k+j-2})\prod_k(1+zq^{k-1})}{\prod_{k,j}(1-zq^{k-1}e^{i\theta_j})(1-zq^{k-1}e^{-i\theta_j})} - 1, \tag{23}$$

where $1, e^{\pm i\theta_1}, \dots, e^{\pm i\theta_n}$ are eigenvalues of $g$ and

$$c_\lambda(z,q) = z^{|\lambda|}q^{n(\lambda)}\prod_{x\in\lambda'}\frac{1-q^{n-c(x)}}{1-q^{h(x)}}. \tag{24}$$

We conclude this section with a remark on the connection between the characters and multivariate orthogonal polynomials.

REMARK 3.3. *The irreducible characters of $SO(2n+1)$, written in terms of the real parts of the eigenvalues, correspond to the Jacobi orthogonal polynomials with respect to $f_{1,\frac{3}{2},\frac{1}{2}}$, namely $\{P_\lambda^{1/2,-1/2}\}$. See, for example, Olshanski and Osinenko (2012).*

3.2. *$U(n)$*. The case of $U(n)$ is the simplest. In this case, the Cauchy identity is identical to the Cauchy-Littlewood identity. The irreducible representations of the unitary group $U(n)$ are labeled by the partitions $\lambda$ of arbitrary non-negative integers with at most $n$ parts. For a partition $\lambda$ let $\pi^\lambda$ be the irreducible representation corresponding to $\lambda$ and $\chi_\lambda$ the corresponding character. The Cauchy identity reads

$$\sum_\lambda s_\lambda(x)\chi_\lambda(g) = \prod_{i,j=1}^n \frac{1}{1-x_i y_j},$$

where $s_\lambda$ is the Schur function in the variables $x_1,\ldots,x_n$, and $y_1,\ldots,y_n$ are the eigenvalues of $g$. In fact, Schur functions computed at the eigenvalues coincide with the characters of the unitary group; but, two different symbols are used above to distinguish different roles of the two functions. Setting $x_i = zq^{i-1}$, one has

$$\sum_\lambda c_\lambda(z,q)\chi_\lambda(g) = \prod_{i,j=1}^n \frac{1}{1-zq^{j-1}y_i},$$

because of (20) and (24).

Thus, the test statistics can be defined as

$$\begin{aligned} U_{z,q}^{(N)} &= \frac{1}{N}\sum_{i,j=1}^N \sum_{\lambda\neq 0} c\lambda(z,q)\chi_\lambda(g_i^* g_j) \\ &= \frac{1}{N}\sum_{i,j=1}^N \left(\prod_{l,k=1}^n \frac{1}{1-zq^{l-1}y_k^{i,j}} - 1\right), \end{aligned}$$

where $y_1^{i,j},\ldots,y_n^{i,j}$ are the eigenvalues of $g_i^* g_j$.

3.3. *$Sp(2n)$*. The irreducible representations of the symplectic group $Sp(2n)$ are labeled by partitions $\lambda$, of non-negative integers, with at most $n$ parts (see Proposition 3.1.20 in Goodman and Wallach (2009, ch. 3)). Let $\chi_\lambda$ be the irreducible character corresponding to $\lambda$. Given independent observations $g_1,\ldots,g_N \in Sp(2n)$, and $0 < z < 1$, define

$$T_{C,z}^{(N)} = \frac{1}{N}\sum_{i=1}^N \sum_{j=1}^N K_z^C(g_i, g_j),$$

where

$$K_z^C(g_i,g_j) \doteq \sum_{\lambda\neq 0} z^{|\lambda|}\chi_\lambda(g_i)\chi_\lambda(g_j).$$

A closed from for $K_z^C(g,h)$ can be found using the Cauchy identity for the symplectic group, Theorem 2.7, as follows:

$$K_z^C(g,h) = \frac{(1-z^2)^m \det\left(\frac{1}{(1-zx_iy_j)(1-zx_i^{-1}y_j)(1-zx_iy_j^{-1})(1-zx_i^{-1}y_j^{-1})}\right)}{z^{\binom{m}{2}}\prod_{i<j}\left(y_i+y_i^{-1}-(y_j+y_j^{-1})\right)\prod_{i<j}\left(x_i+x_i^{-1}-(x_j+x_j^{-1})\right)},$$

where $\{x_i^{\pm}\}$ and $\{y_i^{\pm}\}$ are eigenvalues of $g$ and $h$ respectively.

The test statistic analogous to $U_{z,q}^{(N)}$ is defined through

$$U_{z,q}^{(N)} = N\sum_{\lambda\neq 0} c_\lambda(z,q)\|\widehat{\pi}_N(\lambda)\|_F^2,$$

where $c_\lambda(z,q)$ is defined in (24). The Cauchy-Littlewood identity provides a closed form expression.

PROPOSITION 3.4 (The Cauchy-Littlewood identity Weyl (1946), Section 7.8). *Let $\chi_\lambda$ be the irreducible character of $G = Sp(2n)$ and $s_\lambda$ the Schur function of symmetric function theory. Let $g \in G$ with eigenvalues $y_1^{\pm},\dots,y_n^{\pm}$. Then,*

$$\sum_\lambda s_\lambda(x_1,\dots,x_n)\chi_\lambda(g) = \frac{\prod_{k<j}(1-x_kx_j)}{\prod_{k,j}(1-x_ky_j)(1-x_ky_j^{-1})}. \tag{25}$$

Setting $x_i = zq^{i-1}$, one has

$$\sum_\lambda c_\lambda(z,q)\chi_\lambda(g) = \frac{\prod_{i<j}(1-z^2q^{i+j-2})}{\prod_{i,j}(1-zq^{i-1}y_j)(1-zq^{i-1}y_j^{-1})},$$

because of (20) and (24). Therefore, one has the following closed form definition

$$U_{z,q}^{(N)} = \frac{1}{N}\sum_{k,l=1}^{N}\left(\frac{\prod_{i<j}(1-z^2q^{i+j-2})}{\prod_{i,j}(1-zq^{i-1}y_j^{k,l})(1-zq^{i-1}(y_j^{k,l})^{-1})}-1\right),$$

where $\{y_j^{k,l},(y_j^{k,l})^{-1} \mid j=1,\dots,n\}$ are the eigenvalues of $g_kg_l^T$.

3.4. *$SO(2n)$.* The case of $O(2n)$ is more complicated. A $g\in O(2n)$ with $\det g = 1$ has $n$ pairs of conjugate eigenvalues of norm one. An orthogonal matrix $g \in O(2n)$ with $\det g = -1$ has an eigenvalue equal to 1, another one equal to $-1$, and $n-1$ pairs of conjugate eigenvalues of norm one. This

asymmetry is an indication of the subtlety of the theory for $O(2n)$. Focus on the case of $\det g = 1$; that is, $g \in SO(2n)$. The irreducible representations of $SO(2n)$ are indexed by sequences of integers $\lambda = (\lambda_1, \lambda_2, ..., \lambda_n)$ and $\lambda^- = (\lambda_1, \lambda_2, ..., \lambda_{n-1}, -\lambda_n)$, where $\lambda$ is a partition with at most $n$ parts of an arbitrary non-negative integer. The Weyl character formula is as follows. Let $x_1, x_1^{-1}, \ldots, x_n, x_n^{-1}$ are eigenvalues of $g \in SO(2n)$. If $\lambda_n = 0$, then

$$so_\lambda(g) = \frac{\det\left(x_i^{\lambda_j+n-j} + x_i^{-(\lambda_j+n-j)}\right)}{\det\left(x_i^{n-j} + x_i^{-(n-j)}\right)}. \tag{26}$$

If $\lambda_n > 0$, then the character of the irreducible representation corresponding to $\lambda$ is given by

$$so_\lambda(g) = \frac{\det\left(x_i^{\lambda_j+n-j} + x_i^{-(\lambda_j+n-j)}\right) - \det\left(x_i^{\lambda_j+n-j} - x_i^{-(\lambda_j+n-j)}\right)}{2\det\left(x_i^{n-j} + x_i^{-(n-j)}\right)}, \tag{27}$$

and the one corresponding to $\lambda^-$ is given as

$$so_{\lambda^-}(g) = \frac{\det\left(x_i^{\lambda_j+n-j} + x_i^{-(\lambda_j+n-j)}\right) + \det\left(x_i^{\lambda_j+n-j} - x_i^{-(\lambda_j+n-j)}\right)}{2\det\left(x_i^{n-j} + x_i^{-(n-j)}\right)}. \tag{28}$$

Define $\chi_\lambda$ as $so_\lambda$ if $\lambda_n = 0$, and as $so_\lambda + so_{\lambda^-}$ if $\lambda_n > 0$. In fact, $\chi_\lambda$ is the restriction of the irreducible character of $O(2n)$ to $SO(2n)$; it is an irreducible character of $SO(2n)$ if and only if $\lambda_n = 0$. The test analogous to $T_z^{(N)}$ is constructed in terms of $\{\chi_\lambda\}$ as follows

$$T_{D,z}^{(N)} = \frac{1}{N}\sum_{i=1}^{N}\sum_{j=1}^{N} K_z^D(g_i, g_j),$$

where

$$K_z^D(g_i, g_j) \doteq \sum_{\lambda \neq 0} z^{|\lambda|}\chi_\lambda(g_i)\chi_\lambda(g_j),$$

where the sum is over all partitions of an arbitrary positive integer with at most $n$ parts. A closed from for $K_z^D(g,h)$ is given by the Cauchy identity for $SO(2n)$, Theorem 2.9, as follows:

$$K_z^D(g,h) = \frac{\det\left(\frac{1}{1-zx_iy_j} + \frac{1}{1-zx_i^{-1}y_j} + \frac{1}{1-zx_iy_j^{-1}} + \frac{1}{1-zx_i^{-1}y_j^{-1}}\right)}{z^{\binom{m}{2}}\prod_{i<j}\left(y_i + y_i^{-1} - (y_j + y_j^{-1})\right)\prod_{i<j}\left(x_i + x_i^{-1} - (x_j + x_j^{-1})\right)},$$

where $\{x_i^{\pm}\}$ and $\{y_i^{\pm}\}$ are eigenvalues of $g$ and $h$ respectively.

Similarly, define

$$U_{z,q}^{(N)} = N \sum_{\lambda \neq 0} c_\lambda(z,q) \|\widehat{\pi}_N(\lambda)\|_F^2,$$

where $c_\lambda(z,q)$ is defined in (24). The Cauchy-Littlewood identity provides a closed form expression.

PROPOSITION 3.5 (The Cauchy-Littlewood identity Weyl (1946), Section 7.9). *Let $g \in SO(2n)$ with eigenvalues $y_1^{\pm}, \dots, y_n^{\pm}$. For $\chi_\lambda$ defined above and $s_\lambda$ the Schur function, one has*

$$\sum_\lambda s_\lambda(x_1,\dots,x_n)\chi_\lambda(g) = \frac{\prod_{k\le j}(1-x_k x_j)}{\prod_{k,j}(1-x_k y_j)(1-x_k y_j^{-1})}, \tag{29}$$

*where the sum is over all partitions with at most $n$ parts of arbitrary non-negative integers.*

Setting $x_i = zq^{i-1}$, one has

$$\sum_\lambda c_\lambda(z,q)\chi_\lambda(g) = \frac{\prod_{i\le j}(1-z^2 q^{i+j-2})}{\prod_{i,j}(1-zq^{i-1}y_j)(1-zq^{i-1}y_j^{-1})},$$

because of (20) and (24). Therefore, one has the following closed form definition

$$U_{z,q}^{(N)} = \frac{1}{N}\sum_{k,l=1}^{N}\left(\frac{\prod_{i\le j}(1-z^2q^{i+j-2})}{\prod_{i,j}(1-zq^{i-1}y_j^{k,l})(1-zq^{i-1}(y_j^{k,l})^{-1})} - 1\right),$$

where $\{y_j^{k,l}, (y_j^{k,l})^{-1} \mid j = 1,\dots,n\}$ are the eigenvalues of $g_k g_l^T$.

## 4. Alternative distribution.

PROOF OF PROPOSITION 3.5. Proof of this proposition closely follows section 4 of Giné (1975). The key to fact is that $T_z^{(N)}$ can be written as

$$T_z^{(N)} = \frac{1}{N}\int \left|\sum_{i=1}^{N} g(\theta,\theta^{(i)})\right|^2 f_{1,\frac{3}{2},\frac{1}{2}}(d\theta). \tag{30}$$

Assuming (30), Proposition (4.6) of Giné (1975) directly applies and completes the proof. To prove (30), using Theorem 2.1, we can write

$$g(\theta, \phi) = \sum_{\lambda} z^{|\lambda|/2} \chi_\lambda(\theta)\chi_\lambda(\phi).$$

As a consequence we have

$$g(\theta, \theta^{(i)})g(\theta, \theta^{(j)}) = \sum_{\lambda,\rho} z^{|\lambda|+|\rho|/2} \chi_\lambda(\theta)\chi_\lambda(\theta^{(i)})\chi_\rho(\theta)\chi_\rho(\theta^{(j)}).$$

Integrating against $\theta$ yields

$$\begin{aligned}\int g(\theta, \theta^{(i)})g(\theta, \theta^{(j)}) f_{1,\frac{3}{2},\frac{1}{2}}(d\theta) &= \sum_{\lambda,\rho} z^{|\lambda|+|\rho|/2} \chi_\lambda(\theta^{(i)})\chi_\rho(\theta^{(j)}) \int \chi_\lambda(\theta)\chi_\rho(\theta) f_{1,\frac{3}{2},\frac{1}{2}}(d\theta) \\ &= \sum_{\lambda,\rho} z^{|\lambda|+|\rho|/2} \chi_\lambda(\theta^{(i)})\chi_\rho(\theta^{(j)})\delta_{\lambda,\rho} \\ &= \sum_{\lambda} z^{|\lambda|} \chi_\lambda(\theta^{(i)})\chi_\lambda(\theta^{(j)}).\end{aligned}$$

Summing over $i$ and $j$ and dividing by $N$ gives

$$\frac{1}{N}\int [\sum_{i,j} g(\theta, \theta^{(i)})g(\theta, \theta^{(j)})]\nu(d\theta) = \frac{1}{N}\sum_{\lambda} z^{|\lambda|} \sum_{i,j} \chi_\lambda(\theta^{(i)})\chi_\lambda(\theta^{(j)}).$$

Substiting Equation 8 in the main paper yields

$$\frac{1}{N}\int \left|\sum_{i} g(\theta, \theta^{(i)})\right|^2 \nu(d\theta) = \sum_{\lambda} z^{|\lambda|} \left|\frac{1}{N}\sum_{i} \chi_\lambda(\theta^{(i)})\right|^2 = T_z^{(N)},$$

which proves (30) and completes the proof. □

Proof of lemma 4.5. Expand the squared sum and substitute $u$ by its definition to get

$$\begin{aligned}\left|\sum_{i=1}^{N} u(g_i, g)\right|^2 &= \sum_{i,j=1}^{N} u(g_i, g)u(g_j, g) \\ &= \sum_{i,j=1}^{N} \sum_{\lambda,\rho\neq 0} \sqrt{d_\lambda c_\lambda(z, q) d_\rho c_\rho(z, q)}\chi_\lambda(g_i g^T)\chi_\rho(g_j g^T).\end{aligned}$$

Integrating over $g$ yields

$$\int \left| \sum_{i=1}^{N} u(g_i, g) \right|^2 \mu(dg) = \sum_{i,j=1}^{N} \sum_{\lambda,\rho \neq 0} \sqrt{d_\lambda c_\lambda(z,q) d_\rho c_\rho(z,q)} \left( \int \chi_\lambda(g_i g^T) \chi_\rho(g_j g^T) \mu(dg) \right).$$

Theorem (4.5) in Chapter 2 of Bröcker and tom Dieck (1985) proves that

$$\int \chi_\lambda(g_i g^T) \chi_\rho(g_j g^T) \mu(dg) = \delta_{\lambda,\rho} \frac{\chi_\lambda(g_i g_j^T)}{d_\lambda}.$$

Substitute this into the last equation to get

$$\int \left| \sum_{i=1}^{N} u(g_i, g) \right|^2 \mu(dg) = \sum_{i,j=1}^{N} \sum_{\lambda \neq 0} c_\lambda(z,q) \chi_\lambda(g_i g_j^T),$$

which finishes the proof. □

**5. Randomized Approximate Nearest Neighbor Analysis.** Jones, Osipov and Rokhlin (2011) introduced several fast approximate numerical methods for solving fundamental problems in numerical analysis and linear algebra. Examples include approximate algorithms for highly overdetermined linear regression, low-rank matrix approximation, and very high dimensional nearest neighbor analysis. All of these approximate algorithms are based on fast pseudo-random samplers that generate rotation or unitary matrices. The approximate algorithm for nearest neighbor analysis is detailed below.

Given $N$ points $x_1, \ldots, x_N$ in $\mathbb{R}^d$ and a positive integer $k$, the $k-$nearest neighbor problem asks for the list of the $k$ nearest points to each of the points $x_i$. That is, to find a collection of sets $A_i$ such that $|A_i| = k$ and $A_i$ includes the $k$ closest points to $x_i$ among $x_1, \ldots, x_N$ in $\mathbb{R}^d$. The naive algorithm proceeds as follows. Compute all the pairwise distances and for each $i$ find the $k$ points that have smallest distance to $x_i$, resulting in $A_i$. This is an $O(N^3 kd)$ algorithm, which is computationally prohibitive for large $N$. To reduce the computational cost, Jones, Osipov and Rokhlin (2011) suggested a randomized approximate algorithm; for each point $x_i$, instead of searching for the nearest neighbors among all other point, focus the search on a smaller set of *suspects*, $A_i$, that have high probability of being among the $k-$nearest neighbors of $x_i$. Assuming $A_i$ contains fraction $\alpha$ of all points and fraction $\beta$ of the $k-$nearest neighbors, computational cost of the search for nearest neighbors is reduced by a multiplicative factor of approximately $\alpha/\beta$, which

can be substantial if $\alpha << \beta$. The algorithm is outlined below; for more details see Jones, Osipov and Rokhlin (2011).

The set of suspects $A_i$ is constructed as follows. First, shift all of the points to place their center of mass at the origin and apply a random orthogonal linear transformation on the resulting collection to get the set of points $B$. Divide all the points into two disjoint sets of roughly equal size; that is, let

$$B_- = \{x \in B \mid x(1) < m_1\} \quad B_+ = \{x \in B \mid x(1) \geq m_1\},$$

where $m_1$ is the median of the first coordinate and $x(i)$ is the $i-$th coordinate of the vector $x$. Let $m_2$ be the median of the second coordinate. Define

$$B_{+-} = \{x \in B_+ \mid x(2) < m_2\} \quad B_{++} = \{x \in B_+ \mid x(2) \geq m_2\}.$$

$B_{-+}$ and $B_{--}$ are defined similarly. Repeat the subdivision by splitting each of the four sets into two sets by using the median of the third coordinate. Proceed until there are $2^L$ sets $B_\sigma$ with between $k$ and $2k$ points in each set. The index $\sigma$ is a word of symbols $+$ and $-$ of length $L$. For each point $x_i \in B_\sigma$ define

$$A_i = \{x \in B_\mu \mid \forall \mu; d(\sigma, \mu) \leq 1\}, \tag{31}$$

where $d(\sigma, \mu)$ is the number of places the words $\sigma$ and $\mu$ disagree. For a fixed number $T$, repeat this process $T$ times to construct the sets of suspects $A_i^t$ for $i \leq N, t \leq T$. Finally, for each $i$ let $A_i = \cup_t A_i^t$. The Algorithm 1 summarizes this.

---

ALGORITHM 1. *Randomized Approximate Nearest Neighbors Search*

**Input**: $x_i, \ldots, x_N \in \mathbb{R}$ and a positive integer $k$.
**Output** A collection of sets $A_i$ consisting suspects for each point $x_i$.
1 Shift all the points to make origin the center of mass.
2 For $t = 1, \ldots, T$ repeat 3 through 5:
3 Choose a random orthogonal linear transformation $\Theta$, and replace $x_i$ with $\Theta(x_i)$ for all $i = 1, \ldots, N$.
4 Construct $2^L$ boxes $B_\sigma$ as described above.
5 For each $x_i$ define the set $A_i^t$ via (31).
6 Define $A_i = \cup_t A_i^t$.
7 Return $\{A_i \mid i = 1, \ldots, N\}$.

---

OBSERVATION 5.1. *We carried out the approximate nearest neighbor search, described in Algorithm 1, for $N = 10^4$ data points and $k = 6$ nearest neighbors in dimension $d = 30$. $T$, the number of repetitions was set to $10$. The nearest neighbor search was done with uniform rotations, the fast*

*sampler, and a random rotation generator that is not similar to uniform. The non-uniform sampler was based on the QR decomposition of a matrix $X$ with independent entries distributed according to $U[1, 2]$ instead of Gaussian distribution. It is not hard to numerically detect that this sampler is not uniform. For example, the trace does not behave similar to the uniform case; it appears to be normally distributed with a non-zero mean.*

*The algorithms based on the uniform sampler and the new sampler outperformed the one using the non-uniform sampler by 5%. The results are summarized in Table 1.*

TABLE 1. *Empirical percentage of true nearest neighbors discovered*

| Sampler: | Uniform sampler | The new sampler | Non-uniform sampler |
|---|---|---|---|
| Percentage: | 0.71 | 0.71 | 0.66 |

*This suggest that in potential applications uniformity of the rotations might affect the performance of the method significantly.*

**6. A trace test.** It is a well-known fact due to Diaconis and Mallows (1986) that the trace of a uniformly distributed orthogonal matrix is approximately normally distributed, see Diaconis (1987). One can use this fact to construct a test for uniformity as follows. Choose a uni-variate test of fit for the standard normal distribution. Given data $g_1, \ldots, g_N \in O(n)$, compute $\mathrm{tr}(g_1), \ldots, \mathrm{tr}(g_N)$ and apply your favorite test of normality to test if $\mathrm{tr}(g_i)$ is normally distributed.

We carried out the trace test on the Kac's random and the product of random reflections, aiming to numerically confirm the existing theory about the mixing-times.

First consider the Kac's walk. Results of Oliveira (2009) assert that the mixing time in Wasserstein distance is of order $n^2$, possibly multiplied by logarithmic factor. In each experiment, data consists of $N = 200$ observations of $n = 51$ dimensional rotation matrices based on different number of steps of the walk. The trace test is formally carried out by applying the chi-square test of normality and the Anderson-Darling test to the traces. The results are shown in Table 2. The chi-square test shows that the Kac's walk

TABLE 2. *p-values corresponding to Kac's walk*

| # of steps | 100 | 150 | 200 | 250 | 300 | 350 | 400 | 450 | 500 |
|---|---|---|---|---|---|---|---|---|---|
| $\chi^2$-test | $\ll$1e-15 | $\ll$1e-15 | 2.06e-10 | 6.43e-05 | 6.94e-02 | 3.07e-01 | 2.36e-01 | 1.18e-01 | 6.18e-01 |
| A-D test | $\ll$1e-06 | $\ll$1e-06 | 8.35e-04 | 2.16e-02 | 2.87e-01 | 1.20e-01 | 8.19e-01 | 4.35e-01 | 7.66e-01 |

does not mix before 250 steps. It suggests that the mixing might happen between 250 and 300 step. Note that no statistical test of goodness-of-fit

can provide an upper-bound on the mixing time, because, if the null is not rejected it doesn't mean that the distribution is close to uniform. The Anderson-Darling test, however, suggests a weaker lower bound: it rejects the null hypothesis of uniformity until 200 steps of the walk, but not for 250 steps.

Remark 6.1. *The mixing-time proposed by theory should be of order* $n^2 \log n \approx 10226$. *However, since the constant for the lower-bound is not known, the actual mixing-time could be much shorter of much longer. The trace test suggests a lower bound of about* 250 *steps.*

The trace test was tried also on the random walk generated by product of random reflections. The setup is the same; $N = 200$ and $n = 51$ for different number of steps. The result is presented in Table 3. Thanks to Diaconis and Shahshahani (1986); Porod (1996); Rosenthal (1994) it is known that the total-variation mixing time is of order $\frac{1}{2}n \log n + cn$. For $n = 51$, $\frac{1}{2}n \log n \approx 100$. The chi-square test clearly indicates that mixing does not happen until 100 steps of the walk, but it does not reject the null hypothesis after 110 steps. Whereas, the Anderson-Darling test shows that the mixing does not happen until 140 steps and it might happen after around 150 steps. That roughly means that $c \geq 1$ in order for the chain to mix.

Table 3. *p-values corresponding to iterated random reflections*

| # of steps | 50 | 75 | 90 | 100 | 110 | 125 | 140 | 150 | 175 | 200 |
|---|---|---|---|---|---|---|---|---|---|---|
| $\chi^2$-test | $\ll$1e-15 | $\ll$1e-15 | $\ll$1e-15 | 1.29e-13 | 1.29e-01 | 6.14e-01 | 3.94e-02 | 7.46e-01 | 1.23e-02 | 4.07e-01 |
| A-D test | $\ll$1e-06 | $\ll$1e-06 | $\ll$1e-06 | $\ll$1e-06 | $\ll$1e-06 | 3.00e-06 | 5.01e-03 | 5.34e-02 | 5.16e-02 | 7.44e-01 |

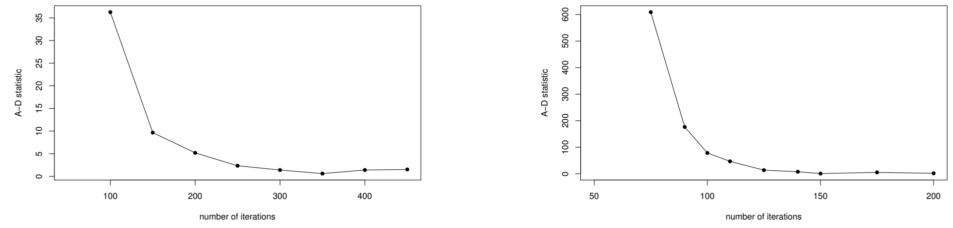


Fig 1. *Values of the Anderson-Darling statistic (left) and the Kolmogorov-Smirnov statistic (right) versus the number of random reflections multiplied.*

The trace test was applied to the new sampler of Jones, Osipov and Rokhlin (2011). For $n = 51$, they suggest that using $\log n \approx 3.93$ iterations suffices for convergence.

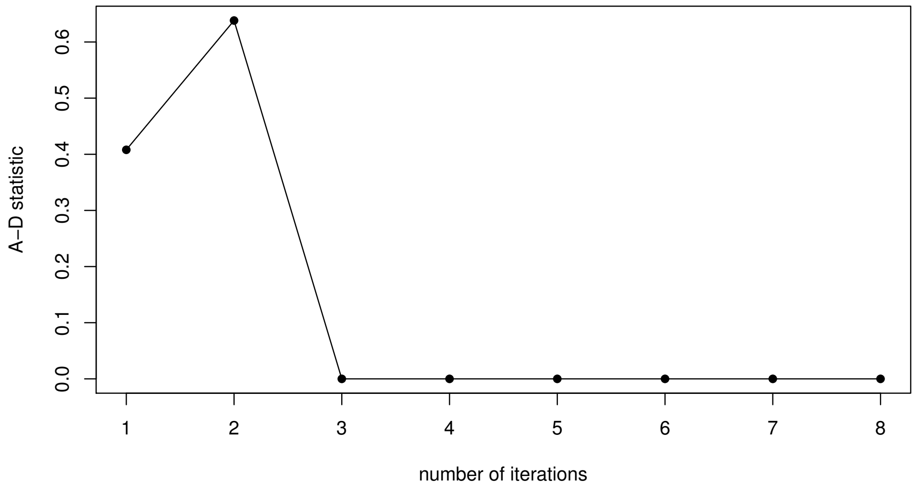


FIG 2. *Values of the Anderson-Darling statistic versus the number of iterations of the new sampler.*

Applying the trace test after only one iteration does not reject the null hypothesis and there is no evidence of departure from the null. The values of the Anderson-Darling statistic are plotted in Figure 2, for different number of iterations of the new sampler. The normal QQ-plot of the traces after a single iteration is illustrated in Figure 3 and the p-values for the chi-square and Anderson-Darling tests are shown in Table 4.

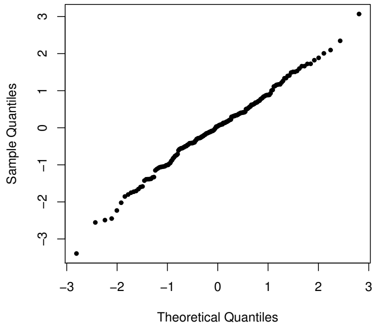


FIG 3. *Normal QQ-plot of the trace for the new sampler*

| # of steps | 1 | 2 |
|---|---|---|
| $\chi^2$-test | 0.58 | 0.87 |
| A-D test | 0.66 | 0.79 |

TABLE 4. *The p-values for the new sampler*

**7. The test based on concentration bands of (Kerkyacharian, Nickl and Picard, 2012).** Per suggestion of the associate editor, the constant in Proposition 4 of (Kerkyacharian, Nickl and Picard, 2012) are computed explicitly using techniques from representation theory. To follow this section, an overall understanding of (Kerkyacharian, Nickl and Picard, 2012) is assumed. For $SO(3)$ the Laplace operator, defined in (Kerkyacharian, Nickl and Picard, 2012), coincides with the Laplace-Beltrami operator. In particular, the eigenspaces are spanned by the matrix coordinates of the irreducible representations. In the case of $SO(3)$, the irreducible representations are labels by non-negative integers $n$. For each $n$ there is an irreducible representation of dimension $2n + 1$, which is given by the action of $SO(3)$ on the spherical harmonics of degree $n$. The corresponding representation is a $(2n + 1) \times (2n + 1)$ matrix; each of the $(2n + 1)^2$ coordinates is an eigenfunction of the Laplace-Beltrami operator, corresponding to a common eigenvalue $\lambda_n$. For any compact classical group the eigenvalues are given, in terms of the dominant weights, by

$$\lambda_j = |j + \rho|_2^2 - |\rho|_2^2, \quad j \in \Lambda_+(G),$$

where $\Lambda_+$ is the cone of dominant weights. See section 2.1 in (Corsi, Haus and Procesi, 2015) for more details. Also, (Goodman and Wallach, 2009), Proposition 3.1.19, describes $\Lambda_+(SO(2l + 1))$ explicitly.

For $SO(3)$ this yields $\lambda_n = n(n + 1)$. Let $\pi_n$ be the irreducible representation corresponding to $n$. Then, $\{\sqrt{2n+1}\pi_n^{i,j} \mid 1 \leq i, j \leq 2n + 1\}$ is an orthonormal basis for the eigenspace corresponding to $\lambda_n$. Following the arguments of section 2.6 in (Kerkyacharian, Nickl and Picard, 2012), we have

$$\begin{aligned} L_n(x, y) &= \sum_{i,j} (2n + 1)\pi_n^{i,j}(x)\pi_n^{i,j}(y) = (2n + 1)\mathrm{Tr}(\pi_n(x)\pi_n(y)^T) \\ &= (2n + 1)\mathrm{Tr}(\pi_n(xy^T)) = (2n + 1)\chi_n(xy^T), \end{aligned}$$

where $\chi_n$ is the character corresponding to $\pi_n$.

$$\begin{aligned}\int_{SO(3)} A_j^2(x,y)dy &= \int_{SO(3)} \left( \sum_{k<2^j} a(\lambda_k/2^{2j})(2k+1)\chi_k(xy^T) \right)^2 dy \\ &= \sum_{k,l<2^j} a(\lambda_k/2^{2j})a(\lambda_l/2^{2j})(2k+1)(2l+1) \int_{SO(3)} \chi_k(xy^T)\chi_l(xy^T)dy \\ &= \sum_{k<2^j} a(\lambda_k/2^{2j})^2(2k+1)^2 \\ &\le \sum_{k<2^j} (2k+1)^2 = (2^j-1)(2^{j+1}-1)(2^{j+1}-3)/3 < \frac{4}{3}2^{3j}.\end{aligned}$$

Similarly,

$$\begin{aligned}\|\phi_{j\eta}\|_\infty &= \sqrt{b_\eta} \sum_{k<2^j} \sqrt{a(\lambda_k/2^{2j})}(2k+1)\chi_k(id) \\ &\le \sqrt{\sum_{k<2^j}(2k+1)^2} < \sqrt{\frac{4}{3}}2^{3j/2}.\end{aligned}$$

In particular, we can take $D_1(SO(3)) = \sqrt{\frac{4}{3}}$ and $D_2(SO(3)) = \frac{4}{3}$.

**8. Asymptotic Properties Under Local Alternatives.** The tests based on $T_z^{(N)}$ and $U_{z,q}^{(N)}$ are consistent against all fixed alternative distributions on the eigenvalues and on the group of all orthogonal matrices, respectively. This is a desirable property, but it is of more interest to investigate the power of the tests in the regime where the alternative approaches the null as the sample size goes to infinity. Formally, it is of interest to analyze the tests when testing $H_0 : \theta = \theta_0$ against $H_1 : \theta = \theta_N$, where $\theta_N$ varies with the sample size $N$. A standard regime is $\theta_N = \theta_0 + h/\sqrt{N}$ for a fixed $h \in \Omega$.

It suffices to consider only compact spaces since all the examples in this paper are compact. For a compact space $X$, say $X = SO(2n+1)$, the space of square-integrable functions on $X$, $\mathcal{L}^2(X)$, is a separable Hilbert space. That is, the Hilbert space $\mathbb{H} = \mathcal{L}^2(X)$ has a countable orthonormal basis. Following the notation of Section 3.2.1 in the main paper, let $1 = f_0, f_1, \ldots$ be an orthonormal basis for $\mathbb{H}$.

Let $\{P_h \mid h \in \mathbb{H}\}$ be a family of distributions on $X$, where $P_h$ is absolutely continuous with respect to $P_{h_0}$ with density $p_h$. Given independent observations $x_1, \ldots, x_N$ from $P_h$ consider the local hypothesis testing problem

$H_0 : h = h_0$ against $H_1 : h = h_0 + \theta/\sqrt{N}$. The log-likelihood of the data is

$$L_{N,\theta} = \sum_{i=1}^{N} \log p_{h_0+\theta/\sqrt{N}}(x_i).$$

Under enough regulatory assumptions, the following 'Taylor expansion' holds

$$\log p_{h_0+h}(x) \doteq \ell_{h_0+h}(x) = \langle \nabla_h \ell_{h_0}(x), h \rangle + \frac{1}{2}\langle h, \nabla_h^2 \ell_{h_0}(x) h \rangle + o(\|h\|^2).$$

Moreover, assume that $\nabla_h \ell$ can be expanded as

$$\nabla_h \ell_{h_0}(x) = \sum_{i=1}^{\infty} \widehat{\ell}_{h_0}(i) f_i(x).$$

Under these assumptions the log-likelihood can be written as

$$L_{N,\theta} = \sum_{i=1}^{\infty} \widehat{\ell}_{h_0}(i)\theta_i \left( \frac{1}{\sqrt{N}} \sum_{k=1}^{N} f_i(x_k) \right) + \frac{1}{2}\left\langle \theta, \left( \frac{1}{N} \sum_{k=1}^{N} \nabla_h^2 \ell_{h_0}(x_k) \right) \theta \right\rangle + o(\|\theta\|^2/N).$$

By the central limit theorem and the law of large numbers, one gets

$$L_{N,\theta} \to \sum_{i=1}^{\infty} \theta_i Z_i - \frac{1}{2} \sum_{i=1}^{\infty} \theta_i^2 \widehat{\ell}_{h_0}(i)^2,$$

where $Z_i \sim \mathcal{N}(0, \widehat{\ell}_{h_0}(i)^2)$ and $Z_i$'s are independent. Various statistical questions can be answered asymptotically using this limiting log-likelihood. Le Cam's theory of *asymptotically normal experiments* is the subject that provides a rigorous treatment of these ideas. The basic concepts are introduced below, see Le Cam (2012) for a textbook treatment in full generality and Lehmann and Romano (2006, Chapters 12 & 13) for an exposition to the theory in the case of finite-dimensional parametric families.

First, the notion of a Gaussian experiment on a Hilbert space $\mathbb{H}$ is reviewed. Identify $\mathbb{H}$ with $\ell_2(\mathbb{R})$ via the orthonormal basis $\{f_i\}$. That is, each $v = \sum v_i f_i \in \mathbb{H}$ is identified with $(v_1, v_2, \ldots) \in \ell_2(\mathbb{R})$. The standard Gaussian process $\boldsymbol{G}_0$ on $\mathbb{H}$ corresponds to $\boldsymbol{Z} = (Z_1, Z_2, \ldots) \in \mathbb{R}^\infty$ such that $Z_i$ are independent standard normal random variables. For $v \in \mathbb{H}$, $\langle \boldsymbol{Z}, v \rangle = \sum_i Z_i v_i$ is distributed as $\mathcal{N}(0, \|v\|^2)$.

The *standard Gaussian shift experiment* on $\mathbb{H}$ is a collection of stochastic processes $\{\boldsymbol{G}_v \mid v \in \mathbb{H}\}$ such that $\boldsymbol{G}_v$ has log-density $\langle \boldsymbol{Z}, v \rangle - \|v\|^2/2$ with respect to $\boldsymbol{G}_0$. That is, $\boldsymbol{Z} \in \mathbb{R}^\infty$ is distributed according to $\boldsymbol{G}_v$ if and only if $Z_i$ are independent random variables and $Z_i \sim \mathcal{N}(v_i, 1)$. In other words it is

a shift of the standard Gaussian process with a vector $v$, therefore carrying the name *Gaussian shift experiment.* In particular, if $\boldsymbol{Z} \sim \boldsymbol{G}_v$ and $u \in \mathbb{H}$ then $\langle \boldsymbol{Z}, u\rangle = \sum_i Z_i u_i$ is distributed as $\mathcal{N}(\langle v, u\rangle, \|u\|^2)$.

The heuristic Taylor expansion sketched above allows one to deduce asymptotic optimality properties for relatively large class of problems from optimality properties of the limiting Gaussian shift experiments. Formal justification of such an expansion needs new definitions. A sequence of probability measures $Q_n$ is called *contiguous* with respect to another sequence $P_n$ if $\lim P_n(E_n) = 0$ implies $\lim Q_n(E_n) = 0$. This is an asymptotic version of absolute continuity. For local families considered above, contiguity follow from a form of mean differentiability.

DEFIN 8.1 (Quadratic Mean Differentiability). *The family of distributions $\{P_\theta \mid \theta \in \Omega\}$ is quadratic mean diffrentiable (QMD) at $\theta_0$ if there exists a function $\nu(x \mid \theta_0)$, for all $x \in X$, such that*

$$\int_X \left[\sqrt{p_{\theta_0+h}} - \sqrt{p_{\theta_0}} - \left\langle \nu(x \mid \theta_0), h\right\rangle\right]^2 \mu(dx) = o(\|h\|^2),$$

*as $\|h\| \to 0$. $\nu$ is called the quadratic mean derivative at $\theta_0$.*

REMARK 8.2. *If $p_\theta$ is QMD at $\theta_0$ then $p_{\theta_0+h/\sqrt{N}}$ is contiguous with respect to $p_{\theta_0}$.*

The following lemmas of Le Cam are the key facts allowing for study of asymptoptotically normal experiments.

PROPOSITION 8.3 (Le Cam's first lemma, Lehmann and Romano (2006), Theorem 12.2.3). *Suppose $p_\theta$ is QMD at $\theta_0$ with derivative $\nu$. Let $\eta(x \mid \theta_0) = \nu(x \mid \theta_0)/\sqrt{p_{\theta_0}(x)}$ be the score function and the self-adjoint operator $\mathcal{I}(\theta_0)$, defined through $\mathcal{I}_{ij}(\eta_0) = \mathbb{E}[\langle \eta_i(\cdot \mid \theta_0), \eta_j(\cdot \mid \theta_0)\rangle]$, be the Fisher information at $\theta_0$. Consider the log-likelihood*

$$L_{N,h} = \sum_{i=1}^N \log p_{\theta_0+h/\sqrt{N}}(x_i) - \log p_{\theta_0}(x_i).$$

*Then,*

$$L_{N,h} - \left[\langle h, Z_N\rangle - \frac{1}{2}\langle h, \mathcal{I}(\theta_0)h\rangle\right] = o_{p_{\theta_0}}(1),$$

*where $Z_N$ is defined through*

$$Z_N = \frac{1}{\sqrt{N}} \sum_{i=1}^N \eta(x_i \mid \theta_0).$$

PROPOSITION 8.4 (Le Cam's third lemma, Lehmann and Romano (2006), Theorem 12.3.3). *Suppose $Q_N$ is contiguous with respect to $P_N$. For a random variable $T_N$ and the log-likelihood $L_N$ assume that $(T_N, L_N)$ converges in distribution to $(T, L)$ under $P_N$. Then, for any bounded continuous function $f$*

$$\mathbb{E}_{Q_N} f(T_n, L_n) \to \mathbb{E}[f(T, L)e^L].$$

These facts allow for passing many questions to the limit and for computing the limiting distribution under the alternative; using them, the asymptotic properties of $T_z^{(N)}$ and $U_{z,q}^{(N)}$ are studied in the following sections.

8.1. *Asymptotic admissibility.* The following lemma relates a testing problem under the experiment $\{P_{\theta_0+h/\sqrt{N}} \mid h \in \mathbb{H}\}$ to the limiting Gaussian shift experiment $\{\boldsymbol{G}_h \mid h \in \mathbb{H}\}$, assuming $\{P_\theta\}$ is QMD at $\theta_0$.

PROPOSITION 8.5 (Lehmann and Romano (2006), Theorem 13.4.1). *For a sequence of tests $\phi_N$, let $\boldsymbol{\beta}_N(h)$ be the power of $\phi_N$ against $P_{\theta_0+h/\sqrt{N}}$. Then, for any subsequence $\{n_j\}$ there is a further subsequence $n_{j_k}$ and a test $\phi$ in the limiting experiment such that, for every $h$,*

$$\lim_{N\to\infty} \boldsymbol{\beta}_N(h) = \boldsymbol{\beta}(h),$$

*where $\boldsymbol{\beta}(h)$ is the power of $\phi$ against $\boldsymbol{G}_h$.*

DEFIN 8.6 (Admissibility). *A test $\phi$ is called admissible if for any test $\tilde{\phi}$ such that $\tilde{\boldsymbol{\beta}}(h) \geq \boldsymbol{\beta}(h)$ for every $h$ one has $\phi = \tilde{\phi}$ almost surely.*

The following corollary is an immediate consequence of Proposition 8.5.

COROLLARY 8.7. *Let $\phi_N^0$ be a sequence of test in the experiment $\{P_{\theta_0+h/\sqrt{N}} \mid h \in \mathbb{H}\}$ such that $\phi_N^0$ converges to an admissible test $\phi$ in the limiting experiment $\{\boldsymbol{G}_h \mid h \in \mathbb{H}\}$. Let $\phi_N$ be another sequence of tests such that $\boldsymbol{\beta}_N(h) \geq \boldsymbol{\beta}_N^0(h)$ for every $h$, where $\boldsymbol{\beta}_N$ and $\boldsymbol{\beta}_N^0$ are the power functions of $\phi_N$ and $\phi_N^0$, respectively. Then, $\phi_N$ and $\phi_N^0$ are asymptotically equivalent in the following sense. For any subsequence $n_j$ there exists a further subsequence $n_{j_k}$ such that, for every $h$,*

$$\lim_{k\to\infty} \boldsymbol{\beta}_{n_{j_k}}(h) = \boldsymbol{\beta}(h),$$

*where $\boldsymbol{\beta}(h)$ is the power of $\phi$.*

The last corollary motivates the following definition: a sequence of tests $\phi_N$ in the experiment $\{P_{\theta_0+h/\sqrt{N}} \mid h \in \mathbb{H}\}$ is called *asymptotically admissible* if it converges to an admissible test $\phi$.

The following result of Birnbaum (1955) is a useful tool for proving admissibility in Gaussian shift experiments.

LEMMA 8.8 (Strasser (1985), Theorem 30.4). *Let $C \subset \mathbb{H}$ be a closed convex subset. Then,*

$$\phi(x) = \begin{cases} 1 & \textit{if} \quad x \notin C, \\ 0 & \textit{if} \quad x \in C, \end{cases}$$

*is admissible for the testing problem $h = 0$ against $h \neq 0$ and is uniquely determined by its power function.*

The following corollary is immediate.

COROLLARY 8.9. *The limiting tests based on $T_z$ and $U_{z,q}$ are admissible. Therefore, the tests based on $\{T_z^{(N)}\}$ and $\{U_{z,q}^{(N)}\}$ are asymptotically admissible.*

PROOF. The test based on $T_z$ rejects for $\{\boldsymbol{Z} \in \mathbb{R}^\infty \mid \sum_\lambda z^{|\lambda|} Z_\lambda^2 > c_{z,1-\alpha}\}$. The set

$$C_z = \{\boldsymbol{Z} \in \mathbb{R}^\infty \mid \sum_\lambda z^{|\lambda|} Z_\lambda^2 \leq c_{z,1-\alpha}\}$$

is clearly convex and closed. Thus the assertion follows from Lemma 8.1. Proof for $U_{z,q}$ is similar. □

8.2. *Power calculations under local alternatives.*

8.2.1. *Local power of $T_z^{(N)}$ against finite-dimensional parametric families.* Let $\{f(\cdot \mid \theta) \mid \theta \in \Omega\}$ be a Q.M.D. family of density functions with respect to the eigenvalue distribution induced by the Haar measure, where $\Omega \subset \mathbb{R}^k$ for a fixed $k$. Assume that $f(\cdot \mid \theta_0) = 1$, that is, $\theta_0$ corresponds to $f_{1,\frac{3}{2},\frac{1}{2}}$. Given data $x_1, \ldots, x_N \sim f(\cdot \mid \theta)$ consider testing $H_0 : \theta = \theta_0$ against $H_1 : \theta = \theta_0 + h/\sqrt{N}$ for a fixed $h \in \Omega$. Let $\ell(x \mid \theta) = \log f(x \mid \theta)$ be the *log-likelihood function*, $\eta(x \mid \theta) = \nabla_\theta \ell(x \mid \theta)$ the *score function*, and $\mathcal{I}(\theta) = -\mathbb{E}_\theta \nabla_\theta^2 \ell(x \mid \theta)$ the *Fisher information matrix* at $\theta$. Let $L_N$ denote

the log-likelihood of the data; to use Le Cam's third lemma one needs the asymptotic joint distribution of $(T_z^{(N)}, L_N)$. The log-likelihood is

(32)

$$\begin{aligned} L_N &= \sum_{i=1}^{N} \ell(x_i \mid \theta_0 + h/\sqrt{N}) - \ell(x_i \mid \theta_0) \\ &= \sum_{i=1}^{N} \eta(x_i \mid \theta_0)^T \frac{h}{\sqrt{N}} + \frac{1}{2N} h^T \nabla_\theta^2 \ell(x_i \mid \theta_0) h + o_p(1) \\ &= \left( \frac{1}{\sqrt{N}} \sum_{i=1}^{N} \eta(x_i \mid \theta_0) \right)^T h + \frac{1}{2} h^T \left( \frac{1}{N} \sum_{i=1}^{N} \nabla_\theta^2 \ell(x_i \mid \theta_0) \right) h + o_p(1). \end{aligned}$$

The score function of QMD families is square-integrable (Le Cam's first theorem); hence, the Peter-Weyl theorem 1.1 yields the following expansion for $\eta(\cdot \mid \theta_0)$:

$$\eta(\cdot \mid \theta_0) = \sum_{\lambda} \widehat{\eta}(\lambda) \chi_\lambda(\cdot), \tag{33}$$

where $\widehat{\eta}(\lambda)$ is the Fourier coefficient $\int \eta(x \mid \theta_0) \chi_\lambda(x) dx$ and the equality is interpreted in $\mathcal{L}^2(f_{1,\frac{3}{2},\frac{1}{2}})$. Substituting (33) in (32) yields

$$L_N = \sum_{\lambda} \widehat{\eta}(\lambda)^T h \left( \frac{1}{\sqrt{N}} \sum_{i=1}^{N} \chi_\lambda(x_i) \right) + \frac{1}{2} h^T \left( \frac{1}{N} \sum_{i=1}^{N} \nabla_\theta^2 \ell(x_i \mid \theta_0) \right) h + o_p(1).$$

As $N \to \infty$, using Law of Large Numbers and Central Limit Theorem, one has

$$\frac{1}{N} \sum_{i=1}^{N} \nabla_\theta^2 \ell(x_i \mid \theta_0) \to -\mathcal{I}(\theta_0)$$
$$\frac{1}{\sqrt{N}} \sum_{i=1}^{N} \chi_\lambda(x_i) \to Z_\lambda,$$

where $Z_\lambda$ are independent standard normal variables. The joint limiting distribution of $(T_z^{(N)}, L_N)$ is

$$(T_z^{(N)}, L_N) \to (T_z, L),$$

where

$$T_z = \sum_{\lambda \neq 0} z^{|\lambda|} Z_\lambda^2 \quad \text{and} \quad L = \sum_{\lambda} (\widehat{\eta}(\lambda)^T h) Z_\lambda - \frac{1}{2} h^T \mathcal{I}(\theta_0) h. \tag{34}$$

Since $f(\cdot \mid \theta)$ is Q.M.D. Le Cam's third lemma implies that the limiting distribution of $T_z^{(N)}$ under $f(\cdot \mid \theta_0 + h/\sqrt{N})$ is given by the following characteristic function

$$\mathbb{E}_h e^{itT_z} = \mathbb{E}_0 e^{itT_z} e^L.$$

Using (34) and independence of $Z_\lambda$'s one gets

$$\mathbb{E}_0 e^{itT_z} e^L = e^{-\frac{1}{2}h^T \mathcal{I}(\theta_0) h} \prod_\lambda \mathbb{E}_0 e^{itz^{|\lambda|} Z_\lambda^2 + (\widehat{\eta}(\lambda)^T h) Z_\lambda}.$$

For each $\lambda$, $Z_\lambda$ is a standard normal variable; therefore,

$$\begin{aligned}
\mathbb{E}_0 e^{itz^{|\lambda|} Z_\lambda^2 + (\widehat{\eta}(\lambda)^T h) Z_\lambda} &= \frac{1}{\sqrt{2\pi}} \int_{\mathbb{R}} e^{itz^{|\lambda|} x^2 + (\widehat{\eta}(\lambda)^T h) x} e^{-x^2/2} dx \\
&= \frac{e^{\frac{(\widehat{\eta}(\lambda)^T h)^2}{2}}}{\sqrt{2\pi}} \int_{\mathbb{R}} e^{itz^{|\lambda|} x^2} e^{-\frac{(x - (\widehat{\eta}(\lambda)^T h))^2}{2}} dx \\
&= e^{\frac{(\widehat{\eta}(\lambda)^T h)^2}{2}} \mathbb{E} e^{itz^{|\lambda|} U_\lambda},
\end{aligned}$$

where $U_\lambda \sim \chi_1^2\left((\widehat{\eta}(\lambda)^T h)^2\right)$ is a non-central chi-square variable on one degree of freedom with non-centrality parameter equal to $(\widehat{\eta}(\lambda)^T h)^2$. Therefore,

$$\begin{aligned}
\mathbb{E}_h e^{itT_z} &= e^{\frac{1}{2}[-h^T \mathcal{I}(\theta_0) h + \sum_\lambda (\widehat{\eta}(\lambda)^T h)^2]} \prod_\lambda \mathbb{E} e^{itz^{|\lambda|} U_\lambda} \\
&= e^{\frac{1}{2}[-h^T \mathcal{I}(\theta_0) h + \sum_\lambda (\widehat{\eta}(\lambda)^T h)^2]} \mathbb{E} e^{it \sum_\lambda z^{|\lambda|} U_\lambda} \\
&= \mathbb{E} e^{it \sum_\lambda z^{|\lambda|} U_\lambda}.
\end{aligned} \tag{35}$$

The last step holds because $h^T \mathcal{I}(\theta_0) h = \sum_\lambda (\widehat{\eta}(\lambda)^T h)^2$, which can be seen as follows:

$$\begin{aligned}
\mathcal{I}(\theta_0) &= \mathbb{E} \eta(x \mid \theta_0) \eta^T(x \mid \theta_0) \\
&= \mathbb{E} \sum_\lambda \widehat{\eta}(\lambda) \chi_\lambda(x) \sum_\lambda \widehat{\eta}(\lambda)^T \chi_\lambda(x) \\
&= \mathbb{E} \sum_{\lambda,\mu} \widehat{\eta}(\lambda) \widehat{\eta}(\mu)^T \chi_\lambda(x) \chi_\mu(x) \\
&= \sum_{\lambda,\mu} \widehat{\eta}(\lambda) \widehat{\eta}(\mu)^T \mathbb{E} \chi_\lambda(x) \chi_\mu(x) \\
&= \sum_\lambda \widehat{\eta}(\lambda) \widehat{\eta}(\lambda)^T,
\end{aligned}$$

where the last equality follows from the orthogonality relations between irreducible characters of the orthogonal group. It follows that

$$h^T \mathcal{I}(\theta_0) h = \sum_{\lambda} h^T \widehat{\eta}(\lambda) \widehat{\eta}(\lambda)^T h$$
$$= \sum_{\lambda} (\widehat{\eta}(\lambda)^T h)^2.$$

The limiting distribution of $T_z^{(N)}$ under the alternative $\theta_0 + h/\sqrt{N}$ is given by (35) as

$$T_z \sim \sum_{\lambda \neq 0} z^{|\lambda|} U_\lambda, \tag{36}$$

where $U_\lambda$ are independently distributed as $\chi_1^2\left((\widehat{\eta}(\lambda)^T h)^2\right)$, a non-central chi-square variable on one degree of freedom with non-centrality parameter equal to $(\widehat{\eta}(\lambda)^T h)^2$.

Let $c_{z,1-\alpha}$ be the asymptotic rejection threshold for $T_z^{(N)}$. That is, using Proposition **??**,

$$\mathbb{P}\left( \sum_{k=1}^{\infty} z^k \chi^2_{p(n,k)} > c_{z,1-\alpha} \right) = \alpha,$$

where $p(n,k)$ is the number of partitions of $k$ into at most $n$ parts and the chi-square variables are independent. Then, the following proposition is an immediate consequence of the argument above.

PROPOSITION 8.10. *Using above notation, the asymptotic power under the local alternative $\theta_0 + h/\sqrt{N}$ is*

$$\boldsymbol{\beta}(h) = \mathbb{P}\left( \sum_{\lambda \neq 0} z^{|\lambda|} U_\lambda > c_{z,1-\alpha} \right),$$

*for $U_\lambda$ defined in (36).*

EXAMPLE 8.11. *For $\theta \in \mathbb{R}$ let $f(x \mid \theta) \propto \exp(\theta \operatorname{tr}(x))$. Then, $\eta(x \mid 0) = \operatorname{tr}(x)$ and $\widehat{\eta}(\lambda) = 0$ for $\lambda \neq (1)$. The local power under $\theta/\sqrt{N}$ is*

$$\boldsymbol{\beta}(\theta) = \mathbb{P}\left( z\ \chi_1^2(\theta^2) + \sum_{k=2}^{\infty} z^k \chi^2_{p(n,k)} > c_{z,1-\alpha} \right).$$

Remark 8.12. *It is not necessary to restrict attention to finite dimensional alternatives for local power calculations. The results of this section can be extended to families with infinite-dimensional parameter space, under mild regularity conditions. In fact, for a Hilbert space $\mathbb{H}$ and a family of distributions $\{f(\cdot \mid \theta) \mid \theta \in \mathbb{H}\}$ the theory of asymptotically normal experiments is similar to the finite-dimensional case. To avoid technical complexity this section has focused on the finite-dimensional case. However, details are carried out for a canonical infinite-dimensional exponential family of alternatives in the next example.*

Example 8.13 (An infinite-dimensional family of alternatives). *For $\Theta = (\theta^\lambda)_\lambda \in \ell^2(\mathbb{R})$ consider the following exponential family*

$$f(x \mid \Theta) \propto e^{\sum_\lambda \theta^\lambda \chi_\lambda(x)}.$$

*Since $\Theta \in \ell^2$, the function $\ell(x \mid \Theta) = \sum_\lambda \theta^\lambda \chi_\lambda(x)$ is well-defined and $\ell(\cdot \mid \Theta) \in \mathcal{L}^2(f_{1,\frac{3}{2},\frac{1}{2}})$. Moreover, for $\Theta = 0$, $\ell(x \mid \Theta) = 0$. Thus $f(x \mid 0)$ corresponds to the Haar measure. Since $\ell(\cdot \mid \Theta)$ is a continuous function and $SO(2n+1)$ is compact, it is bounded. Therefore $f(\cdot \mid \Theta)$ is integrable and defines a probability distribution. Fix $\Theta_0 \in \ell^2(\mathbb{R})$. To compute the local power against $H_1 : \Theta = \Theta_0/\sqrt{N}$, define a one-parameter exponential family as follows. For $t \in \mathbb{R}$ define*

$$\tilde{f}_t(x) = f(x \mid \Theta_0)^t \propto e^{t\sum_\lambda \theta_0^\lambda \chi_\lambda(x)}.$$

*Testing $H_0 : \Theta = 0$ against $H_1 : \Theta = \Theta_0/\sqrt{N}$ is equivalent to testing $\tilde{H}_0 : t = 0$ against $\tilde{H}_1 : t = 1/\sqrt{N}$. The later can be studied using the methods of this section for finite-dimensional alternatives. Indeed, Proposition 8.10 directly applies. The log-likelihood function is $\tilde{\ell}(x \mid t) = t\sum_\lambda \theta_0^\lambda \chi_\lambda(x) - \tilde{\mathcal{A}}(t)$, where $\tilde{\mathcal{A}}(t)$ is the cumulant generating function corresponding to $\tilde{f}_t$. The score function at $t = 0$ is*

$$\tilde{\eta}(x \mid 0) = \sum_\lambda \theta_0^\lambda \chi_\lambda(x).$$

*Expansion of the score function in terms of the characters is already given as*

$$\widehat{\eta}(\lambda) = \theta_0^\lambda.$$

*Invoking Proposition 8.10 yields that the local power is*

$$\mathbb{P}\left(\sum_{\lambda \neq 0} z^{|\lambda|} U_\lambda > c_{z,1-\alpha}\right),$$

*where $U_\lambda$'s are independent and distributed as a non-central chi-square on one degree of freedom with non-centrality parameter equal to $(\theta_0^\lambda)^2$, respectively. In particular, this recovers the previous example in which $f(x \mid \theta) \propto \exp(\theta\,\mathrm{tr}(x))$; here $\theta_0^\lambda = 0$ for $\lambda \neq (1)$ and $\theta_0^{(1)} = \theta$.*

8.2.2. *Local power of $U_{z,q}^{(N)}$ against finite-dimensional parametric families.* Power calculation for $U_{z,q}^{(N)}$ against local alternatives is very similar to that in the previous section. The derivation is only sketched here.

Let $\{f(\cdot \mid \theta) \mid \theta \in \Omega\}$ be a Q.M.D. family of density functions with respect to the Haar measure, where $\Omega \subset \mathbb{R}^k$ for a fixed $k$. Assume that $f(\cdot \mid \theta_0) = 1$; that is, $\theta_0$ corresponds to the Haar measure. Given data $x_1, \ldots, x_N \sim f(\cdot \mid \theta)$, consider testing $H_0 : \theta = \theta_0$ against $H_1 : \theta = \theta_0 + h/\sqrt{N}$ for a fixed $h \in \Omega$. The log-likelihood of the data is

$$L_N = \left(\frac{1}{\sqrt{N}}\sum_{i=1}^N \eta(x_i \mid \theta_0)\right)^T h + \frac{1}{2}h^T\left(\frac{1}{N}\sum_{i=1}^N \nabla_\theta^2 \ell(x_i \mid \theta_0)\right) h + o_p(1).$$

Assuming $\eta(\cdot \mid \theta_0) \in \mathcal{L}^2(SO(2n+1))$, one has

$$\eta(\cdot \mid \theta_0) = \sum_\lambda \sum_{i,j=1}^{d_\lambda} \widehat{\eta}_{ij}(\lambda)\pi_{ij}^\lambda(\cdot)\sqrt{d_\lambda}.$$

Substituting it in the previous equation yields

$$L_N = \sum_{\lambda\neq 0}\sum_{i,j=1}^{d_\lambda} \widehat{\eta}_{ij}(\lambda)^T h \cdot \left(\sum_{i=1}^N \frac{\sqrt{d_\lambda}}{\sqrt{N}}\pi_{ij}^\lambda(\cdot)\right) + \frac{1}{2}h^T\left(\frac{1}{N}\sum_{i=1}^N \nabla_\theta^2 \ell(x_i \mid \theta_0)\right) h + o_p(1).$$

The law of large numbers and central limit theorem give

$$\frac{1}{N}\sum_{i=1}^N \nabla_\theta^2 \ell(x_i \mid \theta_0) \to -\mathcal{I}(\theta_0)$$
$$\frac{\sqrt{d_\lambda}}{\sqrt{N}}\sum_{i=1}^N \pi_{ij}^\lambda(x_i) \to Z_{ij}^\lambda,$$

where $Z_{ij}^\lambda$ are independent standard normal variables and $\mathcal{I}$ is the Fisher information matrix. Therefore, the joint limiting distribution of $(U_{z,q}^{(N)}, L_N)$ under the null is

$$(U_{z,q}^{(N)}, L_N) \to (U_{z,q}, L),$$

where $U_{z,q}$ and $L$ are

$$U_{z,q} = \sum_{\lambda\neq 0} \frac{c_\lambda(z,q)}{d_\lambda} \sum_{i,j=1}^{\lambda} (Z_{ij}^\lambda)^2$$

$$L = \sum_{\lambda\neq 0} \sum_{i,j=1}^{d_\lambda} \widehat{\eta}_{ij}(\lambda)^T h \cdot Z_{ij}^\lambda - \frac{1}{2} h^T \mathcal{I}(\theta_0) h.$$

Using Le Cam's third lemma, the limiting characteristic function of $U_{z,q}$ under the alternative is

$$\mathbb{E}_h e^{itU_{z,q}} = \mathbb{E}_0 e^{itU_{z,q}} e^L,$$

which, similar to (35), simplifies to

$$\mathbb{E}_h e^{itU_{z,q}} = \mathbb{E} e^{it\sum_\lambda \frac{c_\lambda(z,q)}{d_\lambda} \sum_{i,j=1}^{d_\lambda} X_{ij}^\lambda},$$

where $X_{ij}^\lambda$ is a non-central chi-square variable on one degree of freedom with non-centrality parameter equal to $\left(\widehat{\eta}_{ij}(\lambda)^T h\right)^2$ and $\{X_{ij}^\lambda\}$ are mutually independent. Therefore

$$U_{z,q} \cong \sum_\lambda \frac{c_\lambda(z,q)}{d_\lambda} \sum_{i,j=1}^{d_\lambda} X_{ij}^\lambda.$$

Let $c_{1-\alpha}^{z,q}$ be the asymptotic rejection cutoff for the level $\alpha$ test based on $U_{z,q}$. That it,

$$\mathbb{P}\left(\sum_{\lambda\neq 0} \frac{c_\lambda(z,q)}{d_\lambda} \chi^2_{d_\lambda^2} > c_{1-\alpha}^{z,q}\right) = \alpha.$$

The following proposition is a summary of the discussion above:

PROPOSITION 8.14. *Using the notation used above, the asymptotic local power of $U_{z,q}^{(N)}$ against $\theta_0 + h/\sqrt{N}$ is*

$$\mathbb{P}\left(\sum_{\lambda\neq 0} \frac{c_\lambda(z,q)}{d_\lambda} \sum_{i,j=1}^{d_\lambda} X_{ij}^\lambda > c_{1-\alpha}^{z,q}\right).$$

We conclude this section by calculating the local power against a particular infinite-dimensional family of alternatives.

EXAMPLE 8.15. *Similar to Example 8.13, consider the following canonical alternative. For* $\Theta = (\theta_{ij}^{\lambda}) \in \ell^2(\mathbb{R})$ *define*

$$f(x \mid \Theta) \propto \exp\left(\sum_{\lambda \neq 0} \sum_{i,j=1}^{d_\lambda} \theta_{ij}^{\lambda} \frac{\pi_{ij}^{\lambda}(x)}{\sqrt{d_\lambda}}\right).$$

$f(\cdot \mid \Theta)$ *defines a distribution on* $SO(2n+1)$*. Consider the standard local testing problem*

$$H_0 : \Theta = 0 \quad \textit{against} \quad H_1 : \Theta = \Gamma/\sqrt{N}.$$

*Fix* $\Gamma$ *and consider the following embedded one-dimensional exponential family*

$$\tilde{f}_t(x) \propto \exp\left(t \sum_{\lambda \neq 0} \sum_{i,j=1}^{d_\lambda} \gamma_{ij}^{\lambda} \frac{\pi_{ij}^{\lambda}(x)}{\sqrt{d_\lambda}}\right),$$

*and the corresponding testing problem* $H_0 : t = 0$ *against* $H_1 : t = 1/\sqrt{N}$*. Proposition 8.14 implies that the asymptotic local power is*

$$\mathbb{P}\left(\sum_{\lambda \neq 0} \frac{c_\lambda(z,q)}{d_\lambda} X^\lambda > c_{1-\alpha}^{z,q}\right),$$

*where* $X^\lambda$ *is a non-central chi-square variable on* $d_\lambda^2$ *degrees of freedom with non-centrality parameter equal to* $\sum_{i,j=1}^{d_\lambda} \left(\gamma_{ij}^{\lambda}\right)^2$ *and* $\{X^\lambda\}$ *are mutually independent.*

8.3. *Global asymptotic power function against local alternatives.* As shown in sections 3.2 and 4 of the main paper, the goodness-of-fit tests based on $T_z^{(N)}$ and $U_{z,q}^{(N)}$ are consistent in power against all fixed alternatives in the corresponding hypothesis testing problem. However, it is well-known that any test of goodness-of-fit is poor against local (contiguous) alternatives, except possibly in a finite number of directions. Roughly speaking, any test can obtain reasonable power locally against a family of distributions of a fixed finite dimension. This section investigates this phenomenon in the case of $T_z^{(N)}$ and $U_{z,q}^{(N)}$.

8.3.1. *Spectral decomposition of the power function.* Consider the standard local hypothesis setup. Because of Proposition 8.5, one can focus on the limiting Gaussian shift experiment. This section consider the behavior of the power function under local departures from the null. For an arbitrary non-parametric unbiased test $\phi$ in a Gaussian shift experiment, Janssen (1995) has shown that the curvature of the power function admits a principal component decomposition. Focus on $T_z^{(N)}$ and $U_{z,q}^{(N)}$; this will simplify the derivation. For more details and statements in full generality see Janssen (1995).

First consider the test based on $T_z^{(N)}$. Using the notation of section 8.2.1, for a Q.M.D. family of density functions $f(\cdot \mid \theta)$ with $\theta \in \Omega \subset \mathbb{R}^k$, the asymptotic power against the local alternative $H_1 : \theta = \theta_0 + h/\sqrt{N}$ is given by Proposition 8.10 as

$$\boldsymbol{\beta}(h) = \mathbb{P}\left(\sum_{\lambda \neq 0} z^{|\lambda|} U_\lambda > c_{z,1-\alpha}\right),$$

where $U_\lambda$ are independently distributed as non-central chi-square variables on one degree of freedom with non-centrality parameters equal to $(\widehat{\eta}(\lambda)^T h)^2$, respectively. The non-centrality parameters are defined through the Fourier expansion of the score function in the basis of irreducible characters. That is,

$$\eta(\cdot \mid \theta_0) = \sum_{\lambda} \widehat{\eta}(\lambda) \chi_\lambda(\cdot).$$

The rejection cutoff $c_{z,1-\alpha}$ is such that $\boldsymbol{\beta}(\mathbf{0}) = \alpha$. Janssen (1995) considers the second order Taylor expansion of $\boldsymbol{\beta}(th)$ around $t = 0$. This is straightforward in the case of $T_z$ using the above representation of $\boldsymbol{\beta}(h)$. The following lemma of Beran (1975) is the key to deriving such an expansion.

LEMMA 8.16. *Let* $S(\boldsymbol{b}) = \sum_i \sigma_i^2 \chi_i^2(n_i, b_i^2)$, *where* $\boldsymbol{b} = \{b_i \mid i \geq 1\}$, $\sigma_1^2 \geq \sigma_2^2 \geq \cdots > 0$, $\sum n_i \sigma_i^2 < \infty$, $\sum b_i^2 \sigma_i^2 < \infty$, *and* $\{\chi_i^2(n_i, b_i^2) \mid i \geq 1\}$ *are independent non-central chi-square random variables with degrees of freedom equal to* $n_i$ *and non-centrality parameter equal to* $b_i^2$. *Let* $G(x) = \mathbb{P}(S(\boldsymbol{b}) > x)$ *and*

$$G_{i_1,\ldots,i_k}(x) = \mathbb{P}\left(\sum_i \sigma_i^2 \chi_i^2 \left[n_i + 2\sum_{j=1}^{k} \delta(i_j, i)\right] > x\right),$$

*where* $\chi_i^2[\cdot]$ *are independent central chi-square variable with degrees of freedom equal to the argument. Then,*

$$\mathbb{P}\left(S(\boldsymbol{b}) > x\right) = e^{-\sum_i b_i^2/2} \sum_{k=0}^{\infty} (2^k k!)^{-1} \sum_{i_1,\dots,i_k} b_{i_1}^2 b_{i_2}^2 \cdots b_{i_k}^2 G_{i_1,\dots,i_k}(x), \tag{37}$$

*the series converging uniformly in* $x$ *and uniformly over every set of the form* $\{\boldsymbol{b} \mid \sum_i b_i^2 \le c\}$*.*

Using the Lemma 8.16 one has

$$\begin{aligned}
\boldsymbol{\beta}(t\cdot h) &= e^{-\sum_\lambda t^2\cdot(\widehat{\eta}(\lambda)^T h)^2/2} \sum_{k=0}^{\infty} (2^k k!)^{-1} t^{2k} \sum_{\lambda_1,\dots,\lambda_k} \left( \prod_{j=1}^{k} (\widehat{\eta}(\lambda_j)^T h)^2 \right) G_{\lambda_1,\dots,\lambda_k}(c_{z,1-\alpha}) \\
&= (1 - \sum_\lambda t^2 \cdot (\widehat{\eta}(\lambda)^T h)^2/2) \left( G(c_{z,1-\alpha}) + \frac{t^2}{2} \sum_\lambda (\widehat{\eta}(\lambda)^T h)^2 G_\lambda(c_{z,1-\alpha}) \right) + o(t^2) \\
&= G(c_{z,1-\alpha}) + \frac{t^2}{2} \sum_\lambda (\widehat{\eta}(\lambda)^T h)^2 \left[ G_\lambda(c_{z,1-\alpha}) - G(c_{z,1-\alpha}) \right] + o(t^2) \\
&= \alpha + \frac{t^2}{2} \sum_\lambda (\widehat{\eta}(\lambda)^T h)^2 \left[ G_\lambda(c_{z,1-\alpha}) - \alpha \right] + o(t^2).
\end{aligned}$$

Therefore, the curvature of the power function around $t = 0$ is

$$a(h) = \langle T(h), h \rangle,$$

for the positive-definite bi-linear operator

$$T = \sum_\lambda \left[ G_\lambda(c_{z,1-\alpha}) - \alpha \right] \widehat{\eta}(\lambda) \widehat{\eta}(\lambda)^T.$$

This readily gives a principal decomposition of the curvature, with principal components $\{\widehat{\eta}(\lambda)\widehat{\eta}(\lambda)^T\}$ and eigenvalues $G_\lambda(c_{z,1-\alpha}) - \alpha \ge 0$. For a fixed $z$ and $\alpha$, $G_\lambda(c_{z,1-\alpha}) - \alpha$ is a decreasing function of $|\lambda|$. Thus, the highest gain in power is against those alternatives that put most of the load on principal components for smaller $|\lambda|$. More formally, since

$$\sum_\lambda \widehat{\eta}(\lambda)\widehat{\eta}(\lambda)^T = \mathcal{I}(\theta_0),$$

across the set of alternatives $\{h \mid h^T \mathcal{I}(\theta_0) h = c > 0\}$, $T_z$ is more powerful against those with larger values of $(\widehat{\eta}(\lambda)^T h)^2$ for small values of $|\lambda|$. This is illustrated for the infinite-dimensional family of alternatives considered in Example 8.13.

Example 8.17 (Example 8.13 continued). *For the exponential family*

$$f(x \mid \Theta) \propto e^{\sum_\lambda \theta_\lambda \chi_\lambda(x)}$$

*with* $\Theta = (\theta_\lambda)_\lambda \in \ell^2(\mathbb{R})$, *the local power is*

$$\boldsymbol{\beta}(\Theta) = \mathbb{P}\left(\sum_{\lambda \neq 0} z^{|\lambda|} U_\lambda > c_{z,1-\alpha}\right),$$

*where* $U_\lambda$*'s are independent and distributed as a non-central chi-square on one degree of freedom with non-centrality parameter equal to* $(\theta_\lambda)^2$, *respectively. In particular, the following expansion holds around* $t = 0$*:*

$$\boldsymbol{\beta}(t\Theta) = \alpha + \frac{t^2}{2} \sum_\lambda \theta_\lambda^2 \left[G_\lambda(c_{z,1-\alpha}) - \alpha\right] + o(t^2).$$

*Therefore, the principal directions are* $\{e_\lambda \mid \lambda\}$, *where* $e_\lambda \in \ell^2$ *is the vector with a one in the* $\lambda$*-th coordinate and zeros elsewhere. In other words, the principal directions correspond to the irreducible characters of* $SO(2n+1)$. *As a consequence, over the set of alternative* $\{\Theta \mid \|\Theta\|_2 = c > 0\}$, $T_z$ *achieves its highest power against the alternative corresponding to* $\theta_{(1)} = c$ *and* $\theta_\lambda = 0$ *for* $\lambda \neq (1)$.

Theorem 2.1 in Janssen (1995) implies that $T$ is a Hilbert-Schmidt operator and $\|T\|^2 < 2\alpha(1-\alpha)$. This implies that any test performs poor against all alternatives except for a finite dimensional space.

Remark 8.18. *In the case of* $T_z$ *one has*

$$\sum_\lambda \left[G_\lambda(c_{z,1-\alpha}) - \alpha\right]^2 < 2\alpha(1-\alpha).$$

*Thus, for any* $\epsilon > 0$ *there exists a positive integer* $k$ *such that*

$$\sum_{|\lambda| > k} \left[G_\lambda(c_{z,1-\alpha}) - \alpha\right]^2 < \epsilon.$$

*This means that the rate of gain in power against local alternative in all directions is negligible except for possible finitely many directions. A more quantitative version of such a statement is provided in section 8.3.3.*

The results stated above are all local around $t = 0$. They provide information about the rate of change in the power function for different directions of departure form the null for general non-parametric tests of goodness-of-fit. The test based on $T_z$ has a especial structure that allows for further exploration of the ideas of this section. In particular, one can prove previous results globally rather than locally. This is presented below.

For a direction $\boldsymbol{h} = \{h_\lambda\}$, a $t > 0$, and a significance level $\alpha$ define

$$\boldsymbol{\beta}(\alpha, \boldsymbol{h}, t) = \mathbb{P}\left(T_z > c_{z,1-\alpha}\right),$$

where $T_z = \sum_{\lambda \neq 0} z^{|\lambda|} U_\lambda$ for independent non-central chi-square random variables $U_\lambda$ each on one degree of freedom with non-centrality parameters equal to $(t^2 \cdot h_\lambda^2)$, respectively. The cutoff $c_{z,1-\alpha}$ is such that $\boldsymbol{\beta}(\alpha, \boldsymbol{h}, 0) = \alpha$. Let $e_\lambda$ be the principal direction defined above. The following proposition formalizes the arguments above.

PROPOSITION 8.19. *The level $\alpha$ test based on $T_z$ has the properties*

$$\begin{aligned}
&\sup\{\boldsymbol{\beta}(\alpha, \boldsymbol{h}, t) \mid \|\boldsymbol{h}\| = 1\} = \boldsymbol{\beta}(\alpha, e_{(1)}, t),\\
&\boldsymbol{\beta}(\alpha, e_\lambda, t) \leq \boldsymbol{\beta}(\alpha, e_\mu, t) \quad \textit{if} \quad |\lambda| \geq |\mu|,\\
&\lim_{|\lambda| \to \infty} \boldsymbol{\beta}(\alpha, e_\lambda, t) = \alpha.
\end{aligned}$$

This proposition is analogous to that for the Cramer-von Mises test, presented in Neuhaus (1976, Theorem 2.2). The proof is essentially the same and based on the following lemma; see Neuhaus (1976, Proposition 2.1).

LEMMA 8.20. *Let $Z_1$ and $Z_2$ be independent standard normal variables, $\sigma_1 \geq \sigma_2 > 0$, $\rho \in \mathbb{R}$, and $c > 0$. Then,*

$$f(\phi) = \mathbb{P}\left(\sigma_1^2 (Z_1 - \rho \cos\phi)^2 + \sigma_2^2 (Z_2 - \rho \sin\phi)^2 > c\right)$$

*is monotonically non-increasing for $\phi \in [0, \pi/2]$. In other words, the random variables $\sigma_1^2(Z_1 - \rho\cos\phi)^2 + \sigma_2^2(Z_2 - \rho\sin\phi)^2$ are stochastically non-increasing for $0 \leq \phi \leq \pi/2$.*

REMARK 8.21. *An analogous investigation is possible for $U_{z,q}$ which we is not presented here due to similarity to the case of $T_z$. The only major difference is that unlike $T_z$ for which the order of the weights $z^{|\lambda|}$ is clear, the weights $c(z, q)$ for $U_{z,q}$, given in (24), are hard to order. In fact, to the best of our knowledge, ordering of $s_\lambda(1, q, \ldots, q^{n-1})$ are not known in the literature. However, the weights can be computed numerically for a relatively large number of partitions $\lambda$, yielding an ordering of the principal directions for $|\lambda|$ not too large.*

8.3.2. *Asymptotic relative efficiency.* Consider a hypothesis testing problem where two test statistics $\phi_1$ and $\phi_2$ are available. Imagine deciding on which test to use taking into consideration various factors such as the computational cost. One needs a way of comparing performance of the two tests; a classical approach to this problem is through comparison of power functions. For a fixed $\beta \geq \alpha > 0$, let $n_i$ be the sample size needed for the level-$\alpha$ test based on $\phi_i$ to achieve power $\beta$. Roughly speaking, the *Pitman relative efficiency* of the tests is defined as $n_1/n_2$. For instance, a ratio of 2 would indicate that the test based on $\phi_1$ requires twice as many observations as required by $\phi_2$ to achieve the same power at the same level. For two sequences of tests $\phi_1^{(n)}$ and $\phi_2^{(n)}$ the *asymptotic relative efficiency* (ARE) is the limit of the Pitman relative efficiency. That is,

$$\text{ARE} = \lim_{k\to\infty} \frac{n_1^{(k)}}{n_2^{(k)}},$$

assuming that the limit exists. For a more formal treatment and basic properties see (Lehmann and Romano, 2006, Chapter 13).

In a local testing problem the ARE can be computed using the limiting experiments. Focus on the test based on $T_z$ against a fixed alternative $\boldsymbol{h}$. A natural measure of efficiency of $T_z$ in this testing problem is the ARE of $T_z$ with respect to the optimal Neyman-Pearson test

$$\phi^* = \mathbf{1}\left(\left|\sum_\lambda h_\lambda Z_\lambda\right| > \|h\| u_{1-\alpha/2}\right),$$

where $u_{1-\alpha/2}$ is the $1-\alpha/2$-quantile of the standard normal distribution. Following Neuhaus (1976), define $e(\alpha, \boldsymbol{h}, t)$ as the solution $e$ of

$$\boldsymbol{\beta}(\alpha, \boldsymbol{h}, t) = \boldsymbol{\beta}^*_{\boldsymbol{h}}(\alpha, t\sqrt{e}),$$

where $\boldsymbol{\beta}^*_{\boldsymbol{h}}$ is the power function of $\phi^*$. Moreover, define the *local asymptotic relative efficiency* ($\text{ARE}_L$) as

$$e(\alpha, \boldsymbol{h}) = \lim_{t\to 0} e(\alpha, \boldsymbol{h}, t).$$

For a broad range of problems $e(\alpha, \boldsymbol{h}, t)$ indeed equals the Pitman asymptotic efficiency. We only consider $\text{ARE}_L$; the results of this section allow for computation of $\text{ARE}_L$. In particular, it is clear that $\text{ARE}_L$ is closely related

to the curvature of the power function around $t = 0$. In fact, one has

$$\mathrm{ARE}_L(T_z, \boldsymbol{h}) = \frac{\langle \boldsymbol{h}, T(\boldsymbol{h})\rangle}{\|\boldsymbol{h}\|^2 2 f(u_{1-\alpha/2}) u_{1-\alpha/2}} = \frac{\sum_\lambda h_\lambda^2 \left[G_\lambda(c_{z,1-\alpha}) - \alpha\right]}{\|\boldsymbol{h}\|^2 2 f(u_{1-\alpha/2}) u_{1-\alpha/2}},$$

where $f$ is the standard normal density; Janssen (1995, Section 3.2) derives this for a general test. The following corollary is an immediate consequence of Proposition 8.19.

COROLLARY 8.22. *Using the notation of this section, one has*

$$\sup\{e(\alpha, \boldsymbol{h}) \mid \|\boldsymbol{h}\| = 1\} = e(\alpha, e_{(1)})$$
$$e(\alpha, e_\lambda) \leq e(\alpha, e_\mu) \quad \text{if} \quad |\lambda| \geq |\mu|$$
$$\lim_{|\lambda|\to\infty} e(\alpha, e_\lambda) = 0.$$

Similar results hold for $U_{z,q}$ but they are not presented here since the derivation is very similar.

8.3.3. *Dimension of the detectable subspace of alternatives.* Arguments of the previous sections suggest that every omnibus test essentially only uses a finite number of directions. Section 8.3.1 formalizes this phenomenon using the principal component decomposition of the curvature of the power function under infinitesimal departures from the null. This section briefly reviews another formulation of this phenomenon which has a global flavor. Janssen (2000) made the point clear that one can not expect to construct tests with high power, except possibly in a finite-dimensional subspace, by providing specific bounds on the dimension of the subspace. His main result is the following.

PROPOSITION 8.23 (Janssen (2000), Theorem 2.1). *Let $\phi$ be any test for the null hypothesis $P_0$ of the Gaussian shift $\boldsymbol{G}$ with $\mathbb{E}_{P_0}(\phi) = \alpha$ for $0 < \alpha < 1$. For each $\epsilon > 0$ and $K > 0$ there exists a finite dimensional linear subspace $V \subset \mathbb{H}$ with*

$$\sup\{|\mathbb{E}_{P_h}(\phi) - \alpha| : h \in V^\perp, \|h\| \leq K\} \leq \epsilon.$$

*Moreover, the following upper bound*

$$\dim V \leq 1 + \frac{\alpha(1-\alpha)}{\epsilon}(e^{K^2} - 1)$$

*holds independent of the test $\phi$.*

The proof relies on the following lemma.

LEMMA 8.24 (Janssen (2000), Lemma 2.1). *Let $\{h_i\}_{i\in I}$ be an orthonormal system in the parameter space $\mathbb{H}$. For each constant $K > 0$, one has*

$$\sum_{i\in I} (\sup\{|\mathbb{E}_{th_i}(\phi) - \alpha| : |t| \le K\})^2 \le \alpha(1-\alpha)(e^{K^2} - 1). \tag{38}$$

The left hand side of (38) can be written more explicitly in the case of $T_z$ and $U_{z,q}$. Again focus on the case of $T_z$. Using the orthonormal basis $\{e_\lambda\}$ one has

$$\mathbb{E}_{te_\mu}(\phi) = \mathbb{P}\left(\sum_{\lambda\neq 0} z^{|\lambda|} X_\lambda^2 > c_{z,1-\alpha}\right),$$

where $X_\lambda$ are independent standard normal variable except for $\lambda = \mu$. $X_\mu$ is a normal variable with mean $t$ and variance one. In particular, the supremum in (38) is attained for $t = \pm K$ and the result reads as

$$\sum_\lambda \beta_\lambda(K)^2 \le \alpha(1-\alpha)(e^{K^2} - 1),$$

where $\beta_\lambda(K)$ is the gain in power against direction $e_\lambda$. That is,

$$\beta_\lambda(K) = \mathbb{P}\left(\sum_{\mu\neq 0} z^{|\mu|} X_\mu^2 > c_{z,1-\alpha}\right) - \alpha,$$

where $X_\mu$ are independent standard normal variable except for $\mu = \lambda$. $X_\lambda$ is a normal variable with mean $K$ and variance one. The bound can be sharpened in the case of $T_z$ using Lemma 8.16, but it does not contribute to conceptual consequences. The main conceptual consequence is that to test against shrinking alternatives one essentially needs to have a prior knowledge about the alternative, in order to build tests that have high power against it. In particular it, there remains the possibility that, for any fixed sample size, any test will perform poorly against a broad range of alternatives. Therefore, the results of non-parametric tests, when they found no significance, should be interpreted cautiously.

**9. On the sample size and minimax detection rate.** Arias-Castro, Pelletier and Saligrama (2016) recently investigated the **curse of dimensionality** in goodness-of-fit testing problems. The results are described for

the Euclidean space; the case of a manifold is a straightforward extension as mentioned in Arias-Castro, Pelletier and Saligrama (2016). Let $\mathcal{H}$ be a class of real-valued functions on $\mathbb{R}^d$ and $\delta$ a pseudo-metric on $\mathcal{H}$. For $\epsilon > 0$ and a test $\phi$ of the null hypothesis $f_0$, define the worst-case risk of $\phi$, on a sample of size $m$, as

$$R_\epsilon^{(m)}(\phi, f_0, \mathcal{H}) = \mathbb{E}_{f_0}^{(m)}\phi + \sup\{\mathbb{E}_f^{(m)}[1-\phi] \mid f \in \mathcal{H}, \delta(f, f_0) \geq \epsilon\}.$$

The minimax risk is

$$R_\epsilon^{(m)}(f_0, \mathcal{H}) = \inf_\phi R_\epsilon^{(m)}(\phi, f_0, \mathcal{H}).$$

Let $\mathcal{H}_s^d(L)$ be the Hölder class of function $f : [0,1]^d \to \mathbb{R}$ such that $f$ has $\lfloor s \rfloor$ derivatives that satisfies

$$|f^{\lfloor s \rfloor}(x) - f^{\lfloor s \rfloor}(y)| \leq L\|x-y\|^{s-\lfloor s \rfloor}, \quad \forall x, y \in [0,1]^d.$$

Then, Theorem 1 in (Arias-Castro, Pelletier and Saligrama, 2016) states that

$$R_\epsilon^{(m)}(f_0, \mathcal{H}_s^d(L)) \geq 1/2. \quad \text{if } \epsilon < cm^{-2s/(4s+d)},$$

where the constant $c$ depends only on $(d, s, L)$. In particular, if $d \gg \log m$, the upper-bound on $\epsilon$ does not tend to zero as $m$ goes to infinity. Therefore, in order to have non-trivial power against alternatives close to the null, one needs to have $\log m/d > \tilde{c}$. That mean, the sample size needs to be exponential in the dimension. In the case of $SO(51)$, the dimension is 1275. Even a sample size of $N = 50000$ yields $\log(N)/d \approx 0.0085$.

**References.**


Applebaum, D. and Heyer, H. (2014). *Probability on compact Lie groups* **70**. Springer.

Arias-Castro, E., Pelletier, B. and Saligrama, V. (2016). Remember the Curse of Dimensionality: The Case of Goodness-of-Fit Testing in Arbitrary Dimension. *arXiv preprint arXiv:1607.08156*.

Beran, R. (1975). Tail probabilities of noncentral quadratic forms. *The Annals of Statistics* **3** 969–974.

Birnbaum, A. (1955). Characterizations of complete classes of tests of some multiparametric hypotheses, with applications to likelihood ratio tests. *The Annals of Mathematical Statistics* 21–36.

Bröcker, T. and tom Dieck, T. (1985). Elementary Representation Theory. In *Representations of Compact Lie Groups* 64–122. Springer.

Bump, D. (2004). *Lie groups*. Springer.

Corsi, L., Haus, E. and Procesi, M. (2015). A KAM result on compact Lie groups. *Acta Applicandae Mathematicae* **137** 41–59.

DIACONIS, P. (1987). Application of the method of moments in probability and statistics. *Moments in mathematics* **125** 142.

DIACONIS, P. and MALLOWS, C. (1986). On the trace of random orthogonal matrices. *Unpublished manuscript. Results summarized in Diaconis (1990).*

DIACONIS, P. and SHAHSHAHANI, M. (1986). Products of random matrices as they arise in the study of random walks on groups. *Contemp. Math* **50** 183–195.

GINÉ, E. M. (1975). Invariant tests for uniformity on compact Riemannian manifolds based on Sobolev norms. *The Annals of statistics* 1243–1266.

GOODMAN, R. and WALLACH, N. R. (2009). *Symmetry, representations, and invariants* **66**. Springer.

JANSSEN, A. (1995). Principal component decomposition of non-parametric tests. *Probability theory and related fields* **101** 193–209.

JANSSEN, A. (2000). Global power functions of goodness of fit tests. *Annals of Statistics* 239–253.

JONES, P. W., OSIPOV, A. and ROKHLIN, V. (2011). Randomized approximate nearest neighbors algorithm. *Proceedings of the National Academy of Sciences* **108** 15679–15686.

KERKYACHARIAN, G., NICKL, R. and PICARD, D. (2012). Concentration inequalities and confidence bands for needlet density estimators on compact homogeneous manifolds. *Probability Theory and Related Fields* **153** 363–404.

KNOPP, K. (1948). *Theory and application of infinite series.* Hafner New York.

LE CAM, L. (2012). *Asymptotic methods in statistical decision theory.* Springer Science & Business Media.

LEHMANN, E. L. and ROMANO, J. P. (2006). *Testing statistical hypotheses.* Springer Science & Business Media.

MACDONALD, I. G. (1995). *Symmetric functions and Hall polynomials* **354**. Clarendon press Oxford.

MACPHAIL, M. (1941). Cesàro summability of a class of series. *Bulletin of the American Mathematical Society* **47** 483–487.

NEUHAUS, G. (1976). Asymptotic power properties of the Cramér-von Mises test under contiguous alternatives. *Journal of Multivariate Analysis* **6** 95–110.

OLIVEIRA, R. I. (2009). On the convergence to equilibrium of Kac's random walk on matrices. *The Annals of Applied Probability* 1200–1231.

OLSHANSKI, G. and OSINENKO, A. (2012). Multivariate Jacobi polynomials and the Selberg integral. *Functional Analysis and Its Applications* **46** 262–278.

POROD, U. (1996). The cut-off phenomenon for random reflections. *The Annals of Probability* **24** 74–96.

ROSENTHAL, J. S. (1994). Random rotations: characters and random walks on SO (n). *The Annals of Probability* 398–423.

STRASSER, H. (1985). *Mathematical theory of statistics: statistical experiments and asymptotic decision theory* **7**. Walter de Gruyter.

WEYL, H. (1946). *The Classical Groups, Their Invariants and Representations.* Princeton University Press.

WHEELER, M. and ZINN-JUSTIN, P. (2016). Refined Cauchy/Littlewood identities and six-vertex model partition functions: III. Deformed bosons. *Advances in Mathematics* **299** 543–600.
